# Supplementary material for: Data Type Agnostic Visual Sensitivity Analysis
Source: arXiv:2309.03580 source file (2023-09-07)

# Project Info

- Project: Blind Source Separation in Time and Space
- Grant Number: Austrian Science Fund (FWF) P31881-N32
- Principal Investigator: Klaus Nordhausen klaus.k.nordhausen@jyu.fi
- Me: Nikolaus Piccolotto nikolaus.piccolotto@tuwien.ac.at
- **Goal of this study: Investigate interactive visualizations to support tuning parameter selection for Spatial Blind Source Separation**

# Problem Context

- SBSS is a statistical method for analysis of multivariate spatial data
- Finds latent dimensions that are marginally and spatially uncorrelated
- Often correspond to physical processes that generate the data

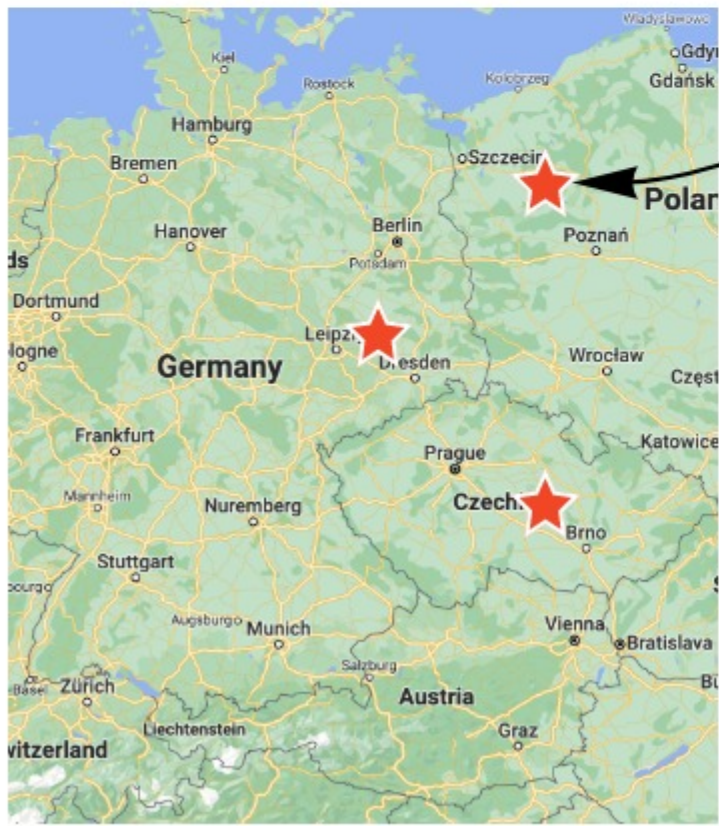

Aluminium: 100 mg/kg  
Barium: 167 mg/kg  
Iron: 20 mg/kg  
Magnesium: 35 mg/kg  
Zinc: 303 mg/kg

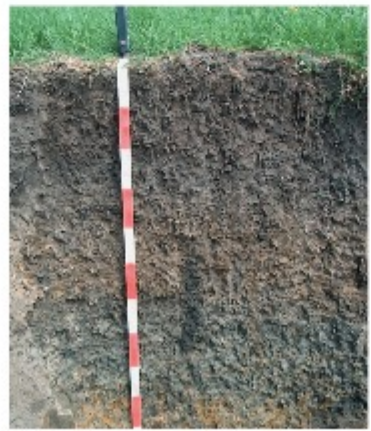

Example: Geochemical measurements

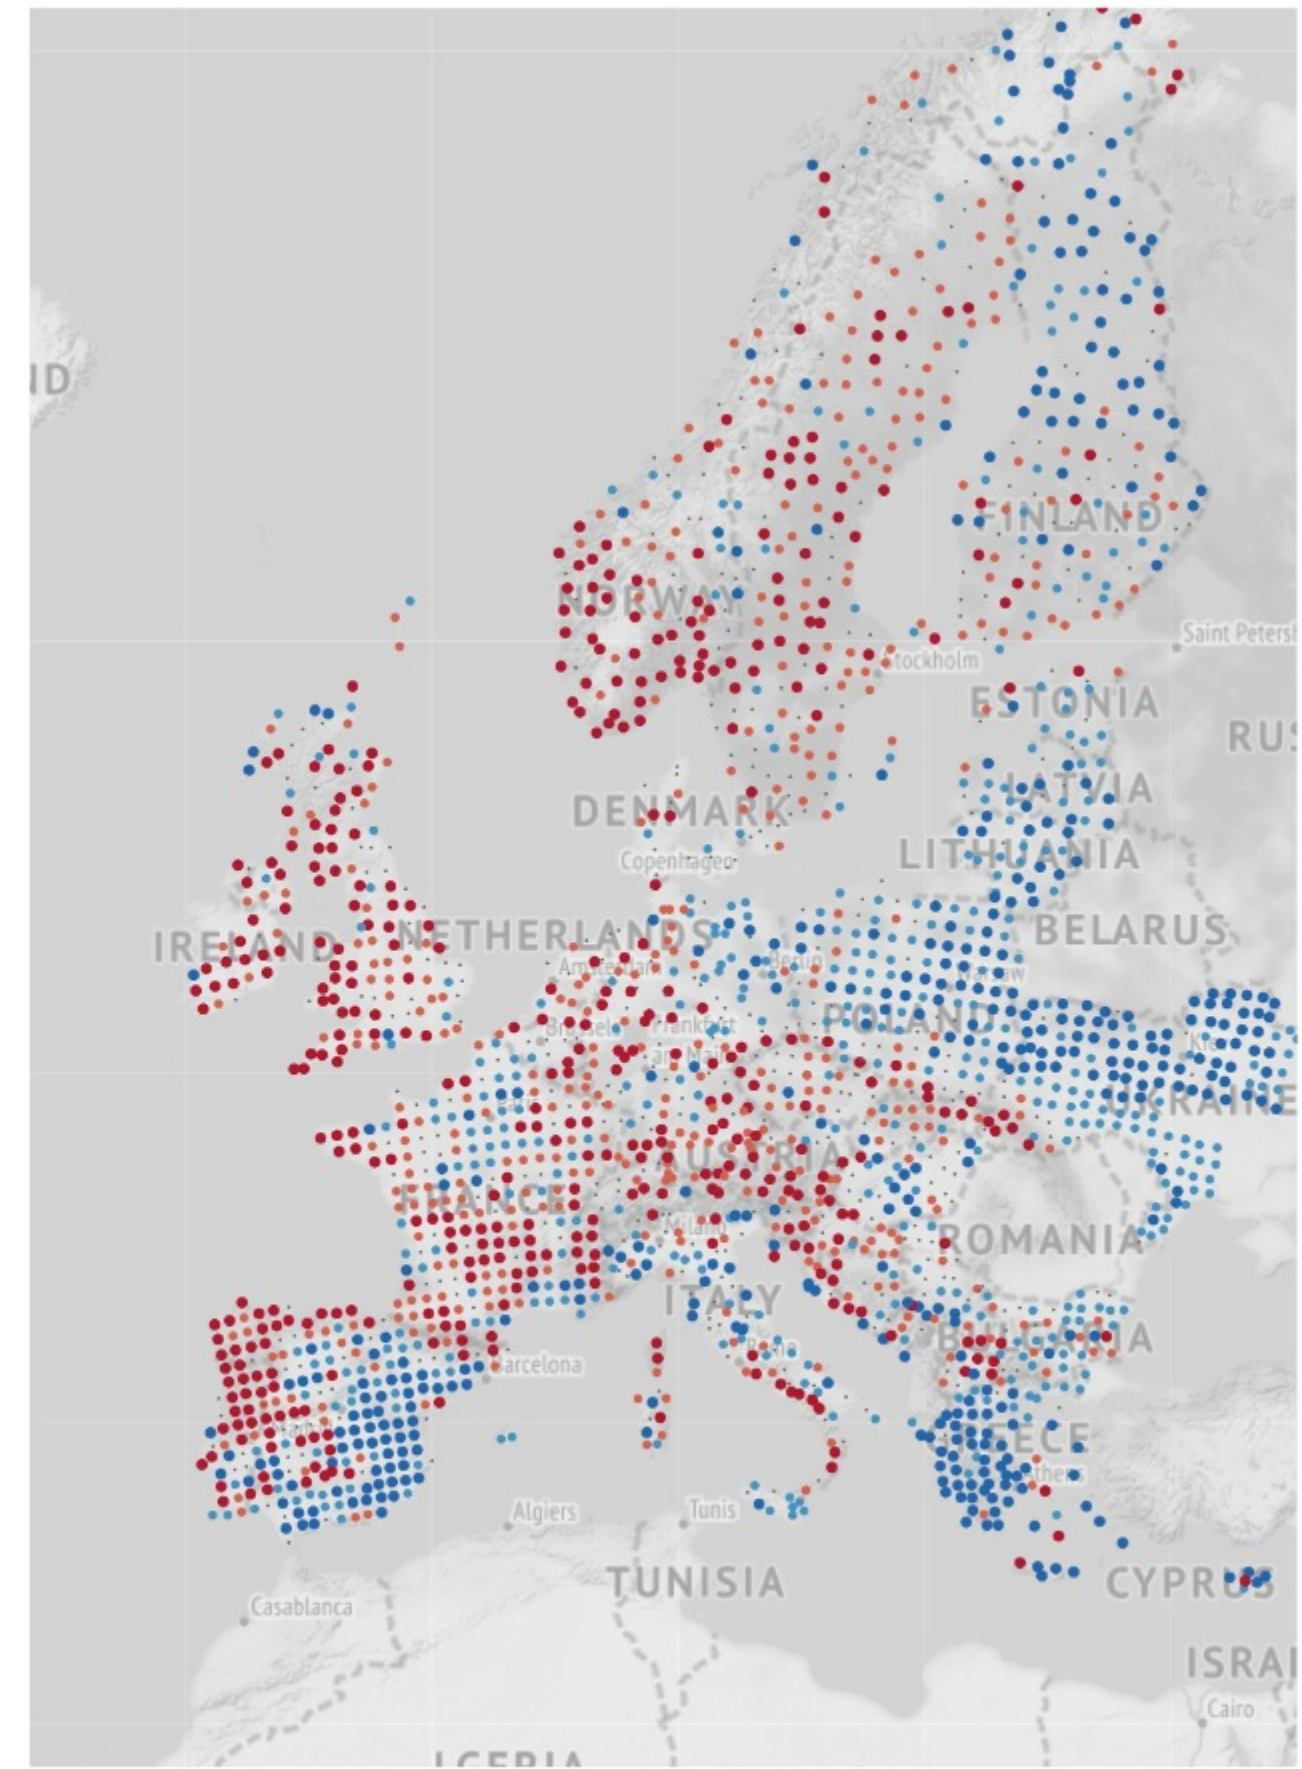

Example latent dimension. Red = high values, blue = low values.

# SBSS Parameters

- Regionalization
  - Partitions the domain into non-overlapping regions
  - Defines "special" areas where variables behave distinctively
- Kernel
  - Composed of one or more concentric rings
  - Defines neighbourhood to consider for calculations

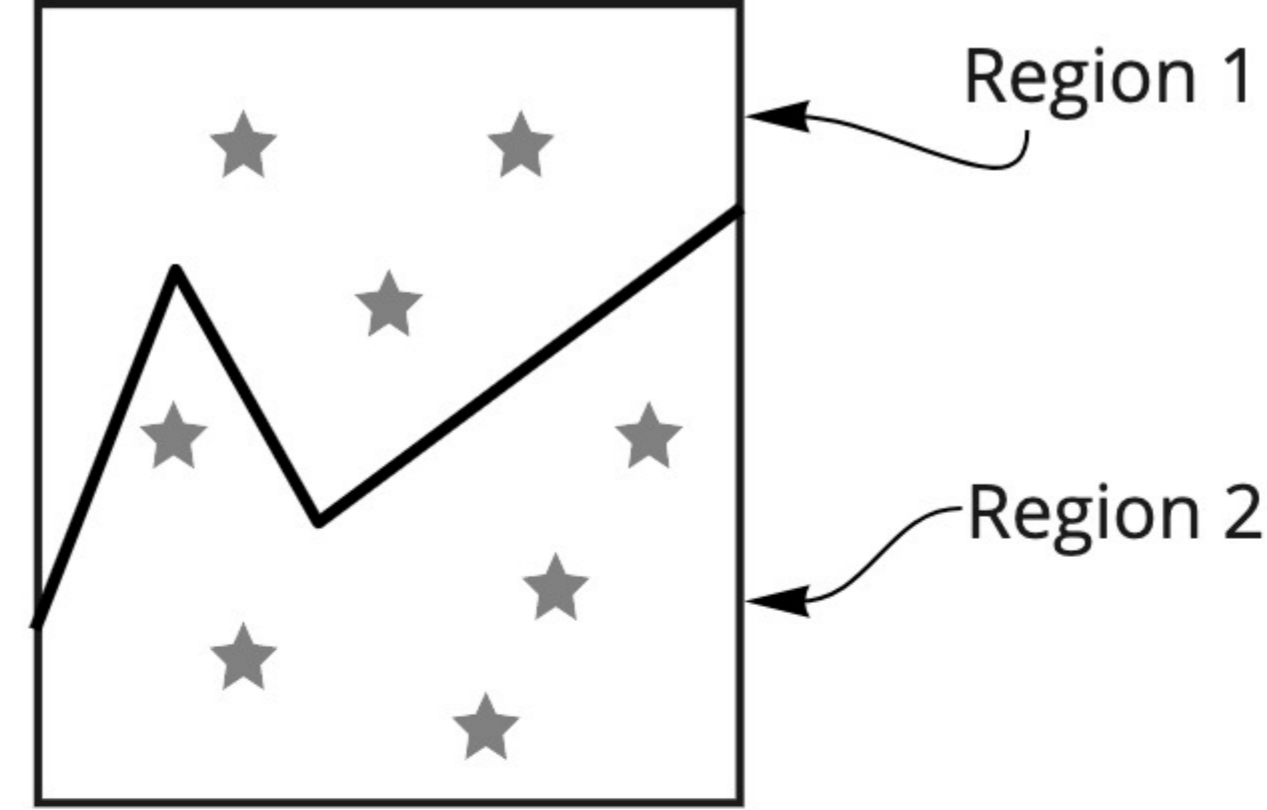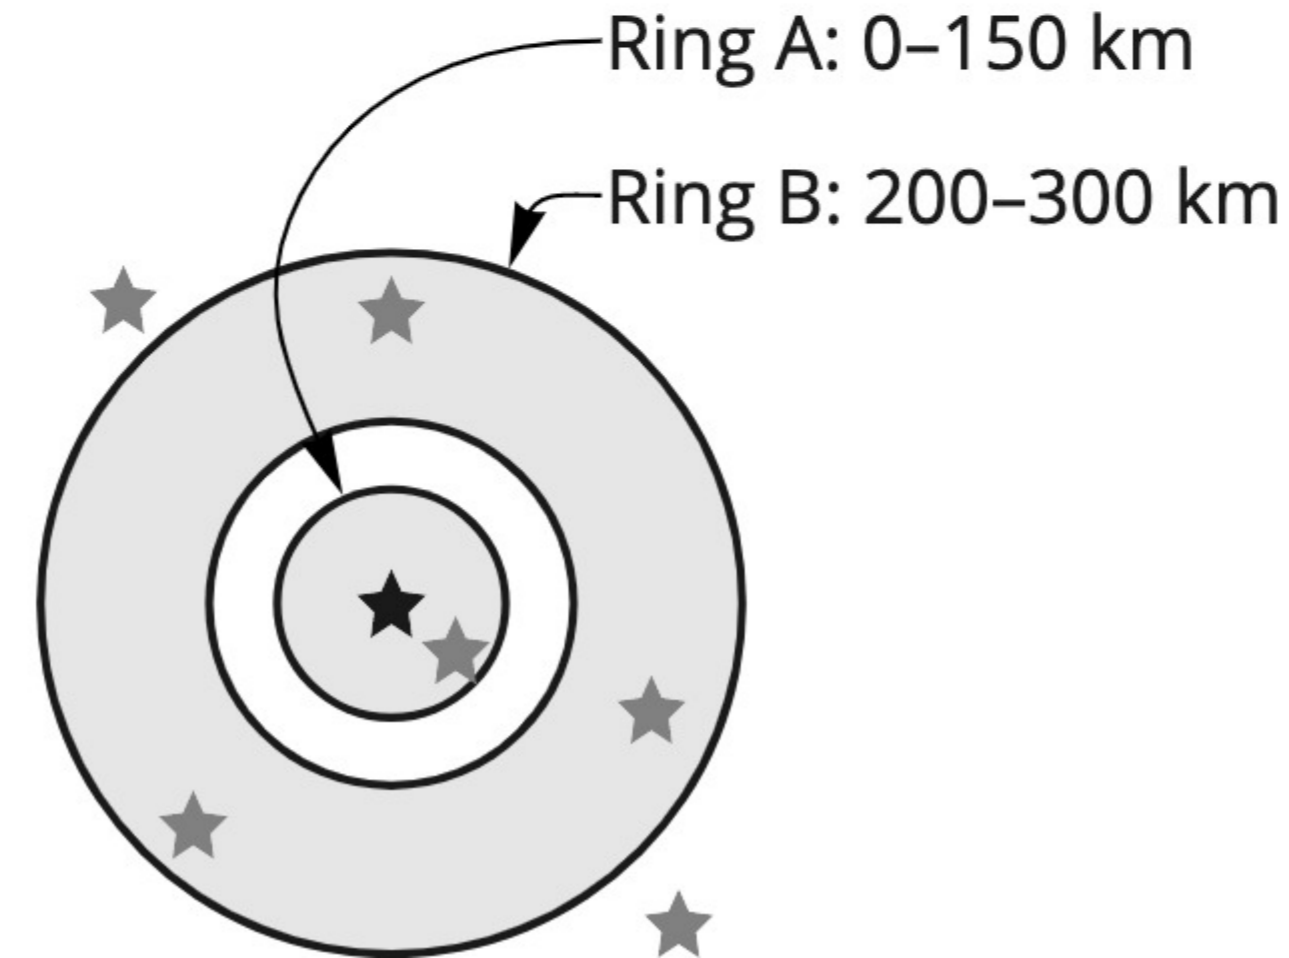

# Sensitivity Analysis

- In simplified terms, the goal of SA is to compare variation in tuning parameters and the model output.
- General reasons
  - Assess importance of parameters
  - Identify stable/sensitive ranges of parameter values

# Sensitivity Analysis

- Large amount of literature on the problem, but underlying model is always numeric, i.e.,  $\mathbf{y} = f(\mathbf{x})$
- This model doesn't fit well to SBSS
- Alternative: Visual analysis
  - PCPs, scatterplots, tilemaps show correlations/dependencies
- These *\*also\** require numeric data
- Our approach: Visual analysis by comparing cluster diameters

# Dissimilarity/Distance measures

- Specialized dissimilarity measures, that quantify (=assign a number to) the similarity of two objects, exist for a lot of data types. For example:

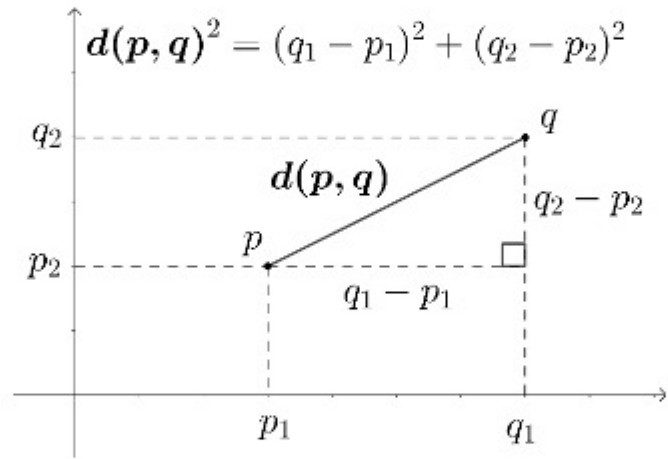

*points in metric space*

| bread | milk | coffee | sugar | coca cola | chocolate | water | jam |
|-------|------|--------|-------|-----------|-----------|-------|-----|
| 1     | 1    | 0      | 0     | 1         | 0         | 0     | 0   |
| 1     | 0    | 0      | 0     | 0         | 0         | 0     | 0   |
| 0     | 1    | 0      | 0     | 0         | 0         | 1     | 0   |
| 1     | 0    | 0      | 1     | 0         | 0         | 0     | 1   |
| 0     | 1    | 1      | 1     | 0         | 0         | 0     | 0   |
| 1     | 0    | 1      | 0     | 0         | 1         | 0     | 0   |
| 0     | 0    | 0      | 0     | 1         | 1         | 0     | 0   |

*boolean vectors (=sets)*

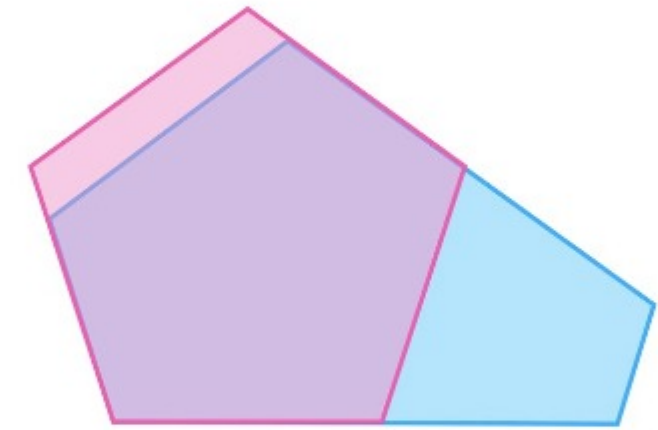

*polygons*

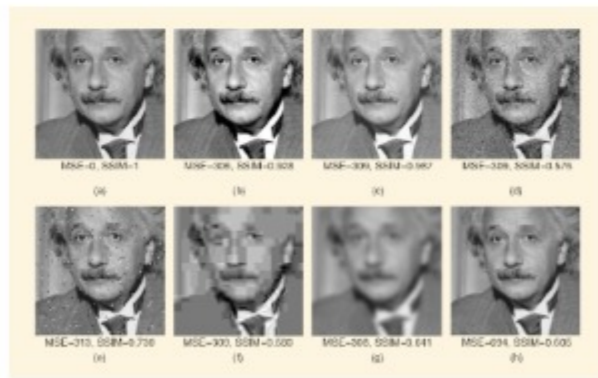

*images*

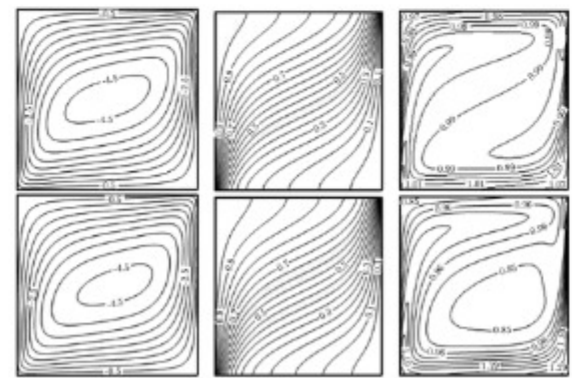

*isocontours*

# The Sensitivity Index

- Based on one-at-a-time sensitivity analysis from literature
- Similar to how you visually compare PCP axes
- Procedure
  - Compute distance matrices and convert values to ranks
  - Index of subset = difference of lowest rank (highest value)

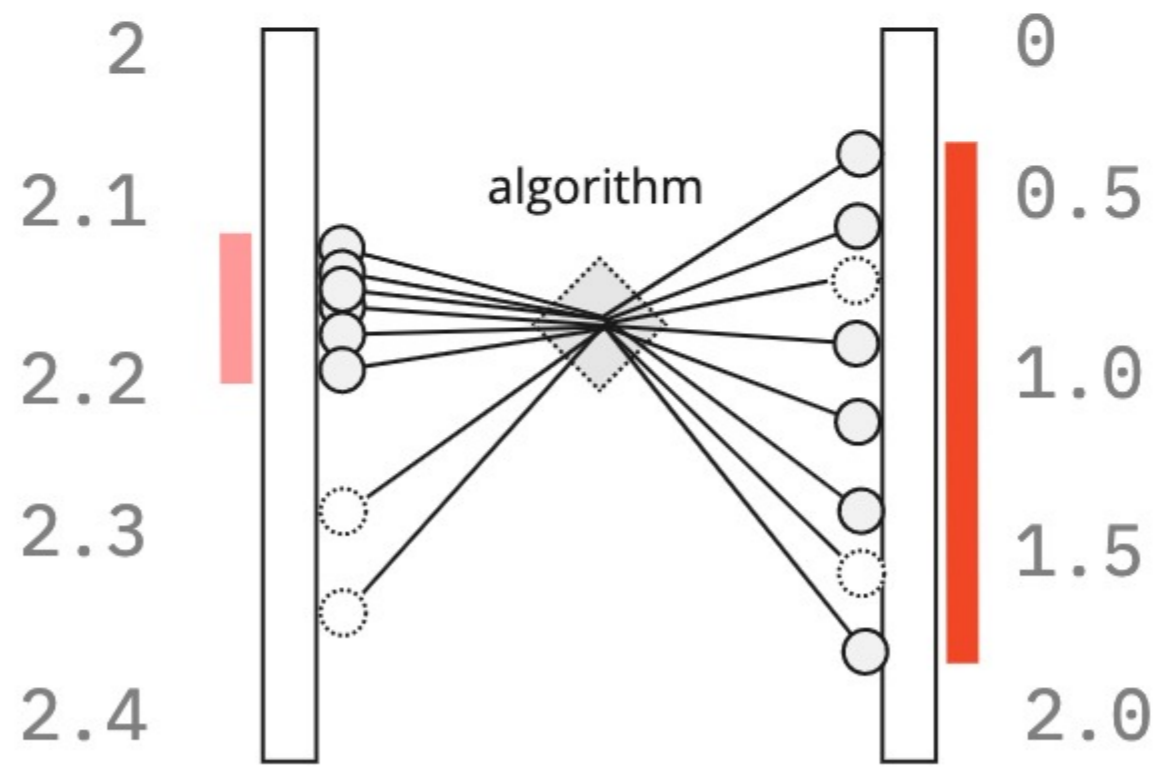

$$d = d_p - d_o = 16 - 1 = 15$$

$\Delta=1 = \text{rank } 16$     *Parameter*

*Output*

$\Delta=1.6 = \text{rank } 1 \text{ of all pairwise distances}$

# The Sensitivity Index

- $d = d_p - d_o \rightarrow$  parameters are this much more/less similar than associated outputs
- Caveats
  - This index only looks at **one parameter at a time**. It does not know about multi-parameter interactions.
  - Its exact meaning (stable/sensitive parameter) has to be inferred in context, as we will see later
  - This index is primarily a simple way to point analyst to interesting data cases
- How to visualize it?

# Dendrogram

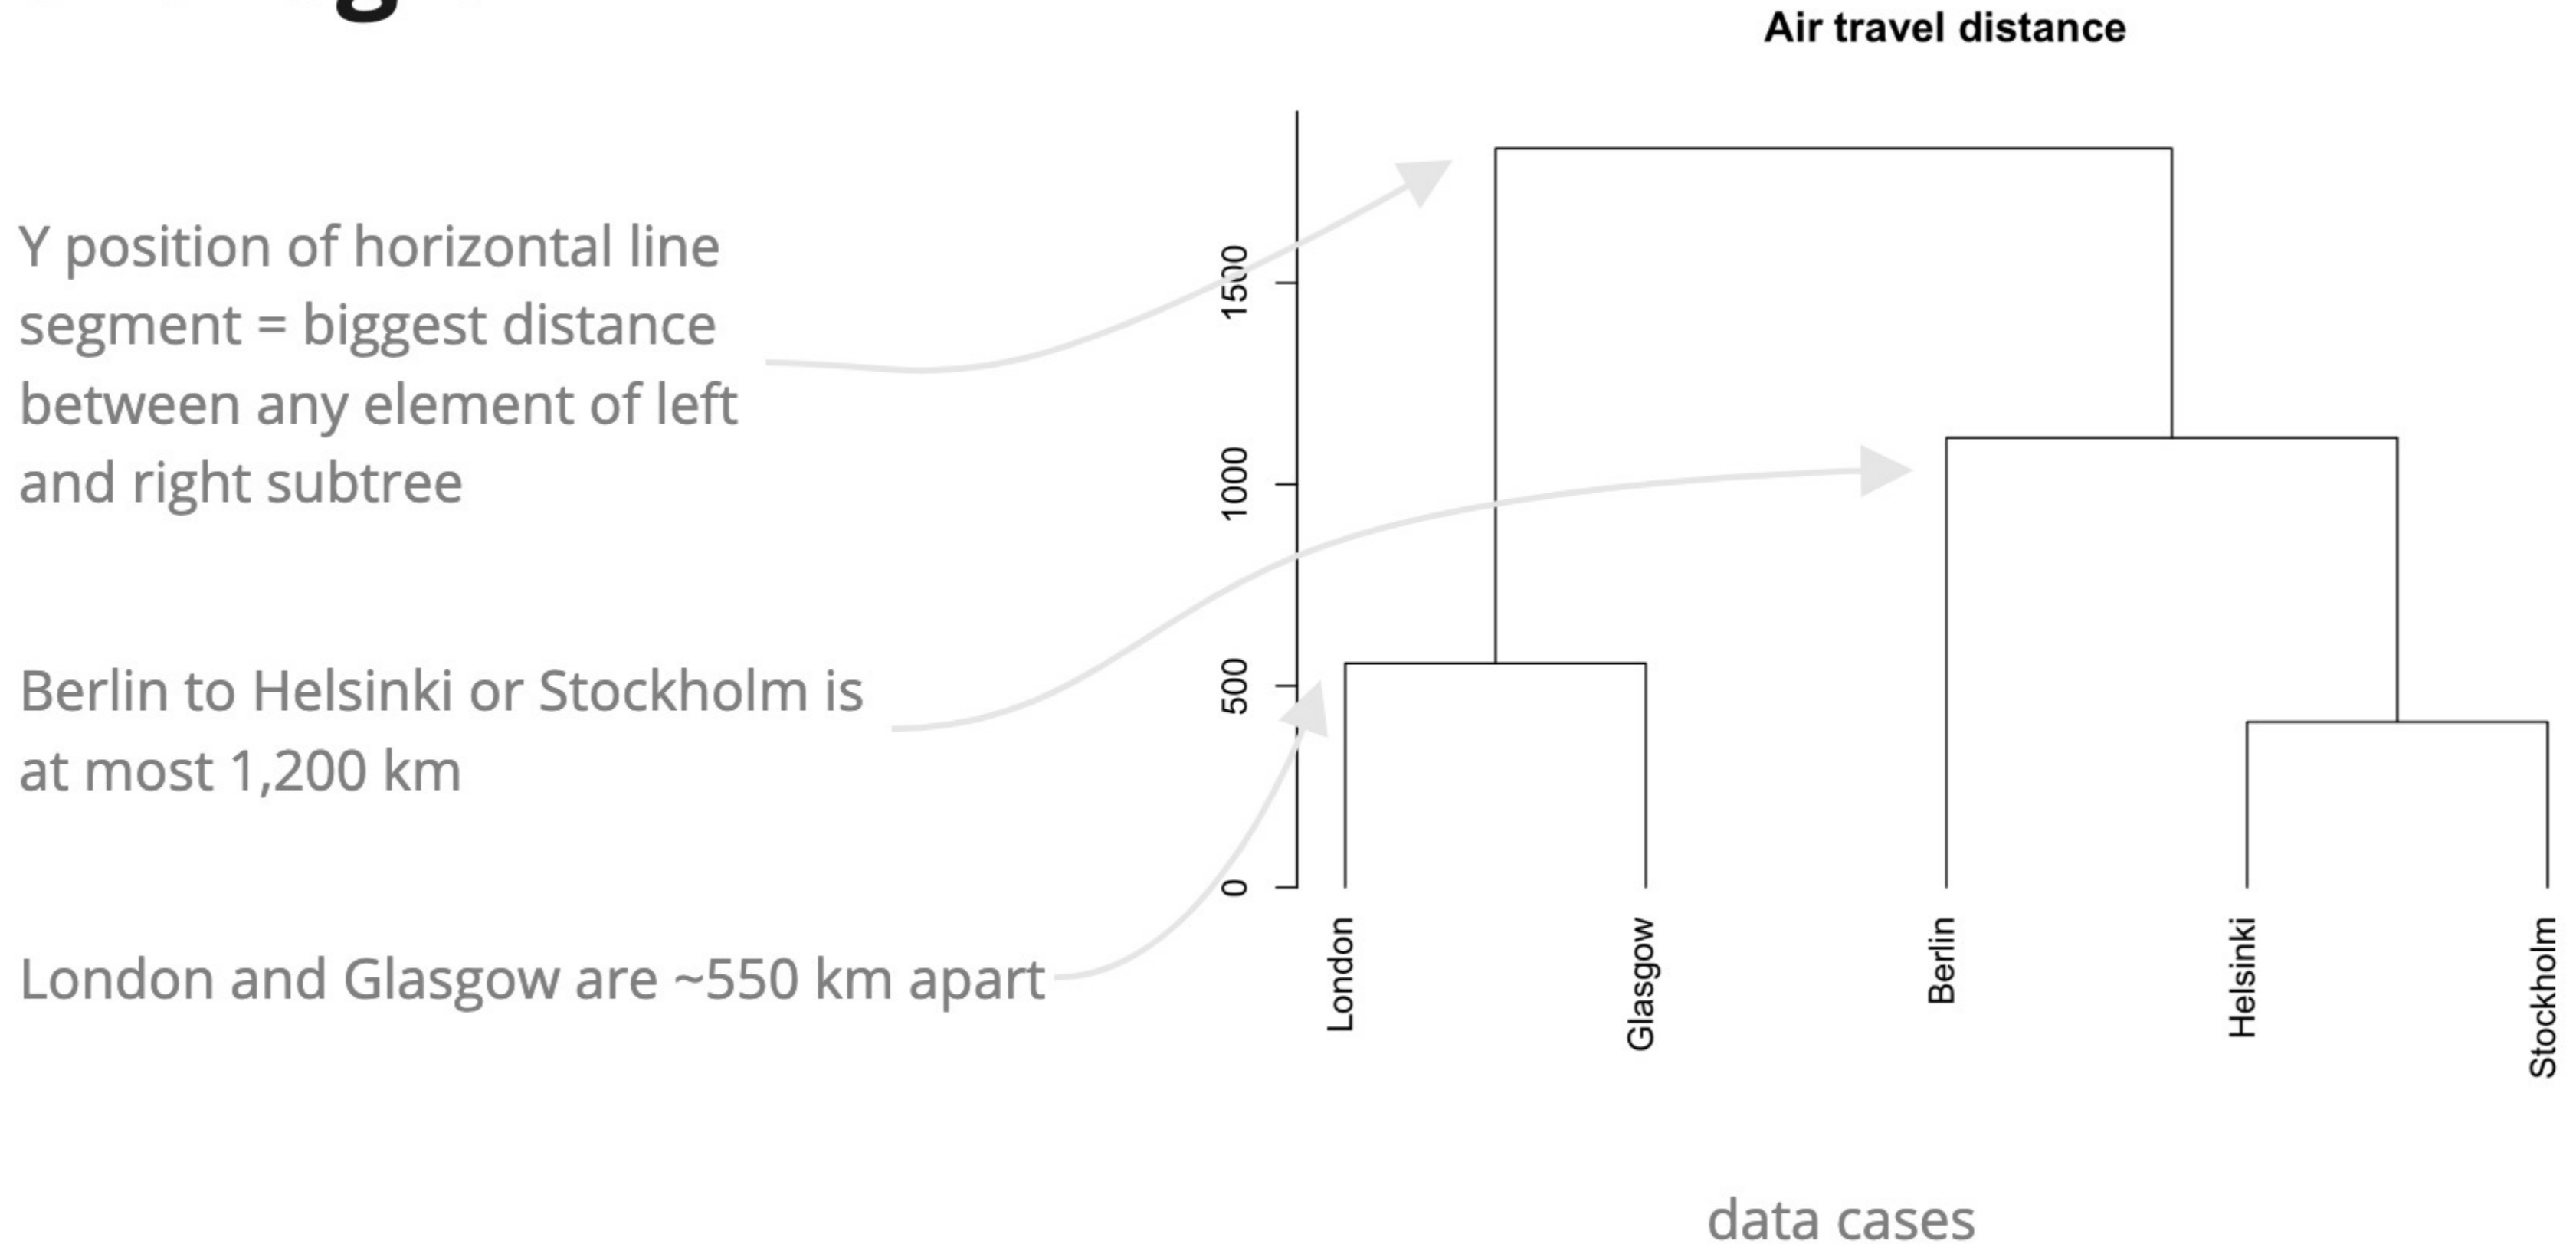

# Dendrogram

- Basic idea here is that SA may be possible by comparing "distances"
- Given this visualization (dendrogram) of similarity A, how to additionally show change when using similarity B?
- Example: Air travel distance vs ground travel distance (no ferries) of 5 European cities

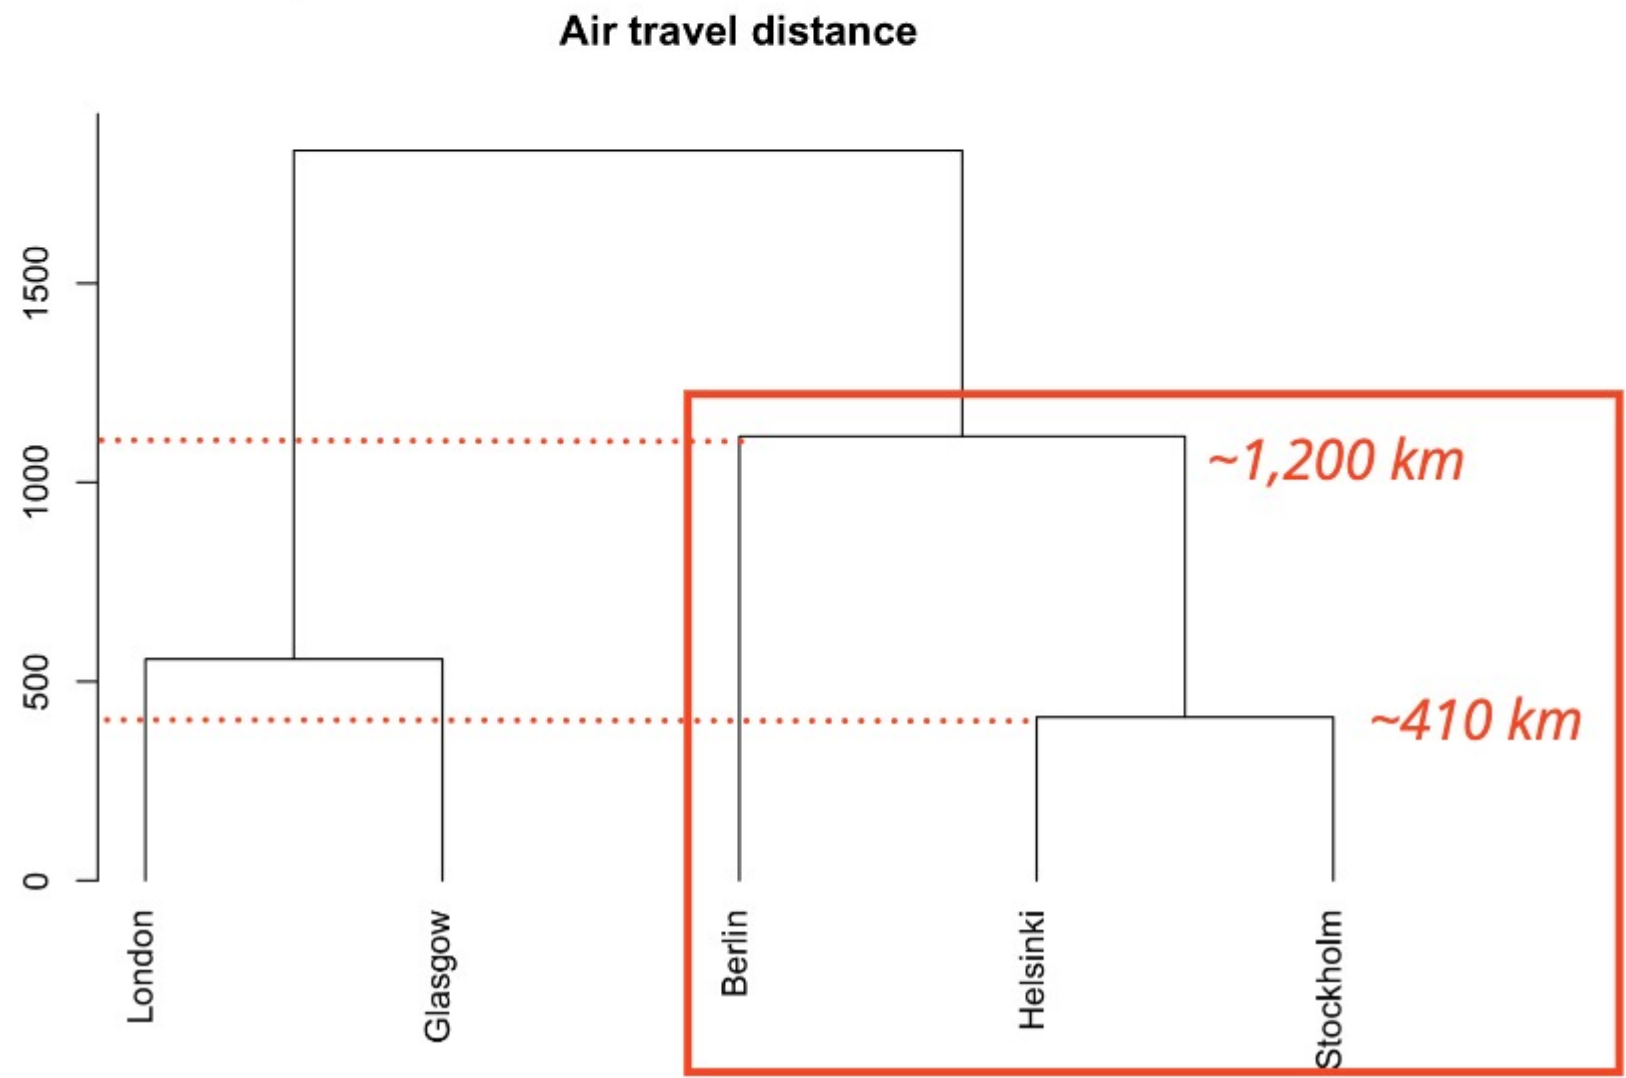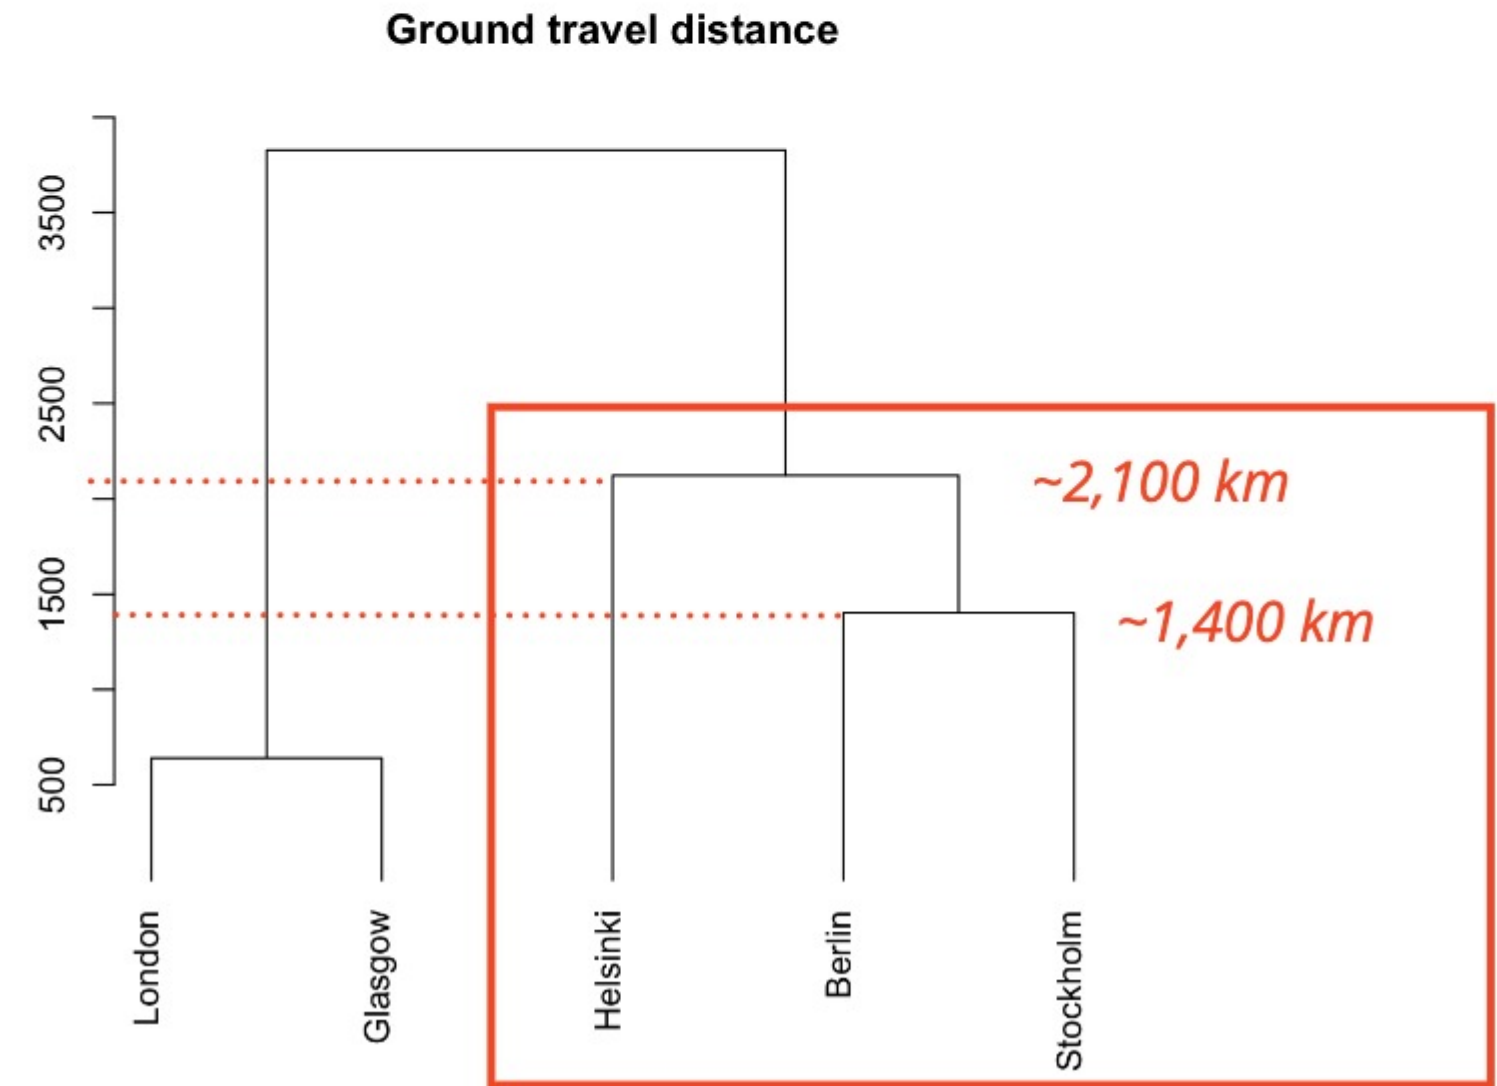

# Discrepancy Dendrogram

- Uses color to encode where the line for data cases would be in a dendrogram with other similarity metric
- (Note: We use ranked/normed distances instead of actual values.)

Air travel distance

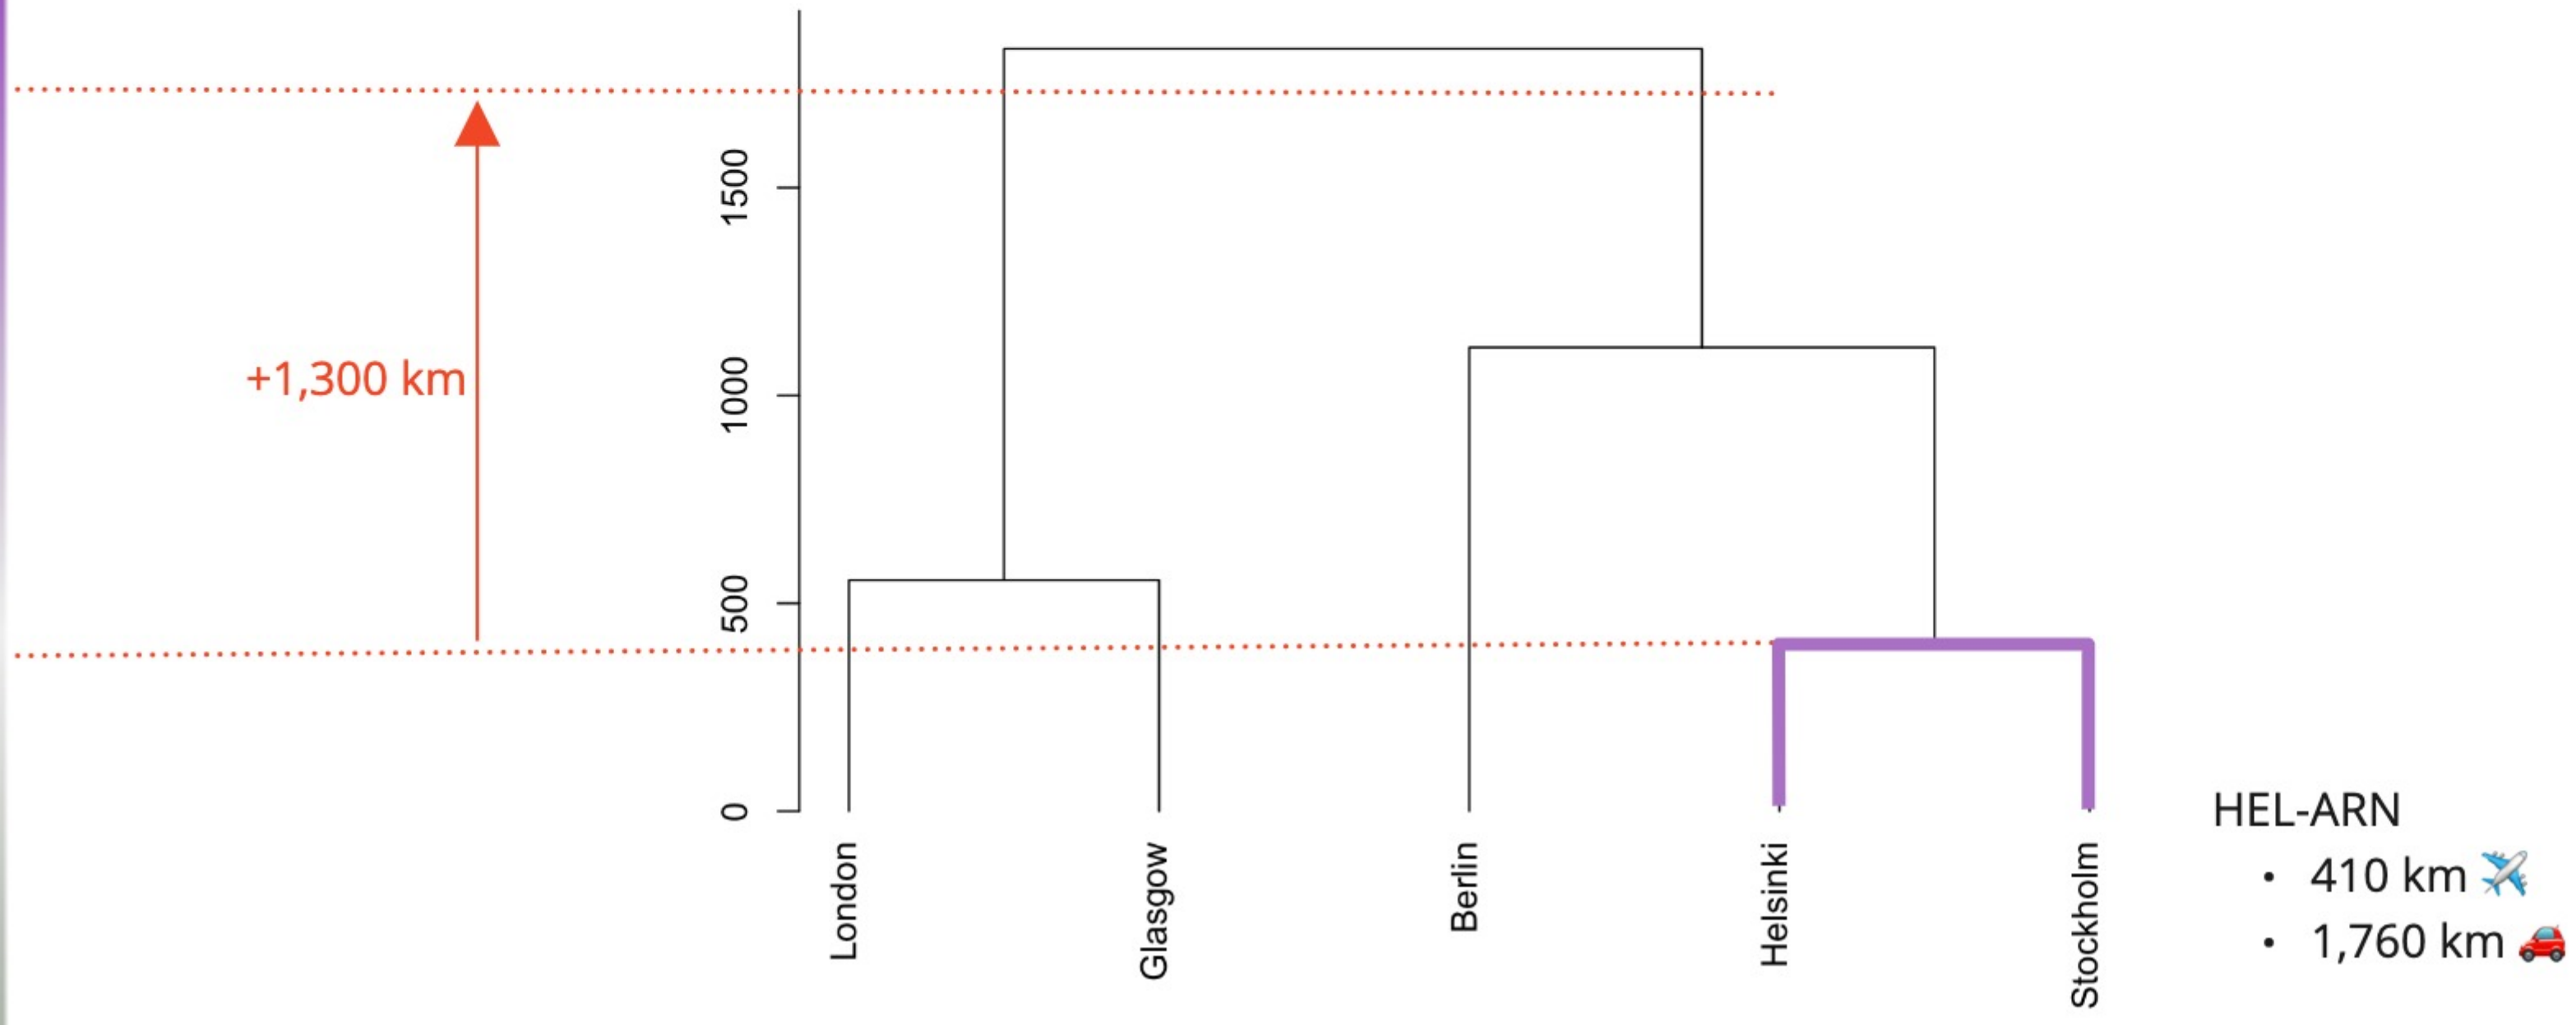

# Discrepancy Dendrogram

- A dendrogram, but lines colored by sensitivity index of the respective subsets of data cases
- Interesting data = colored lines

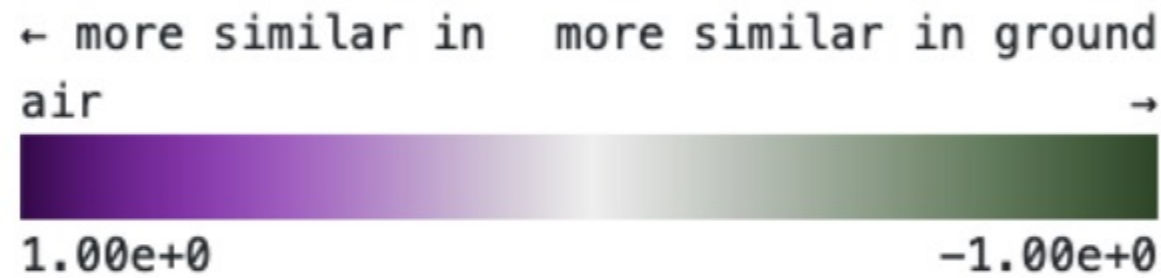

- Low Y: Close in air
- High Y: Far in air
- Green: Closer on ground than in air
- Purple: Further on ground than in air

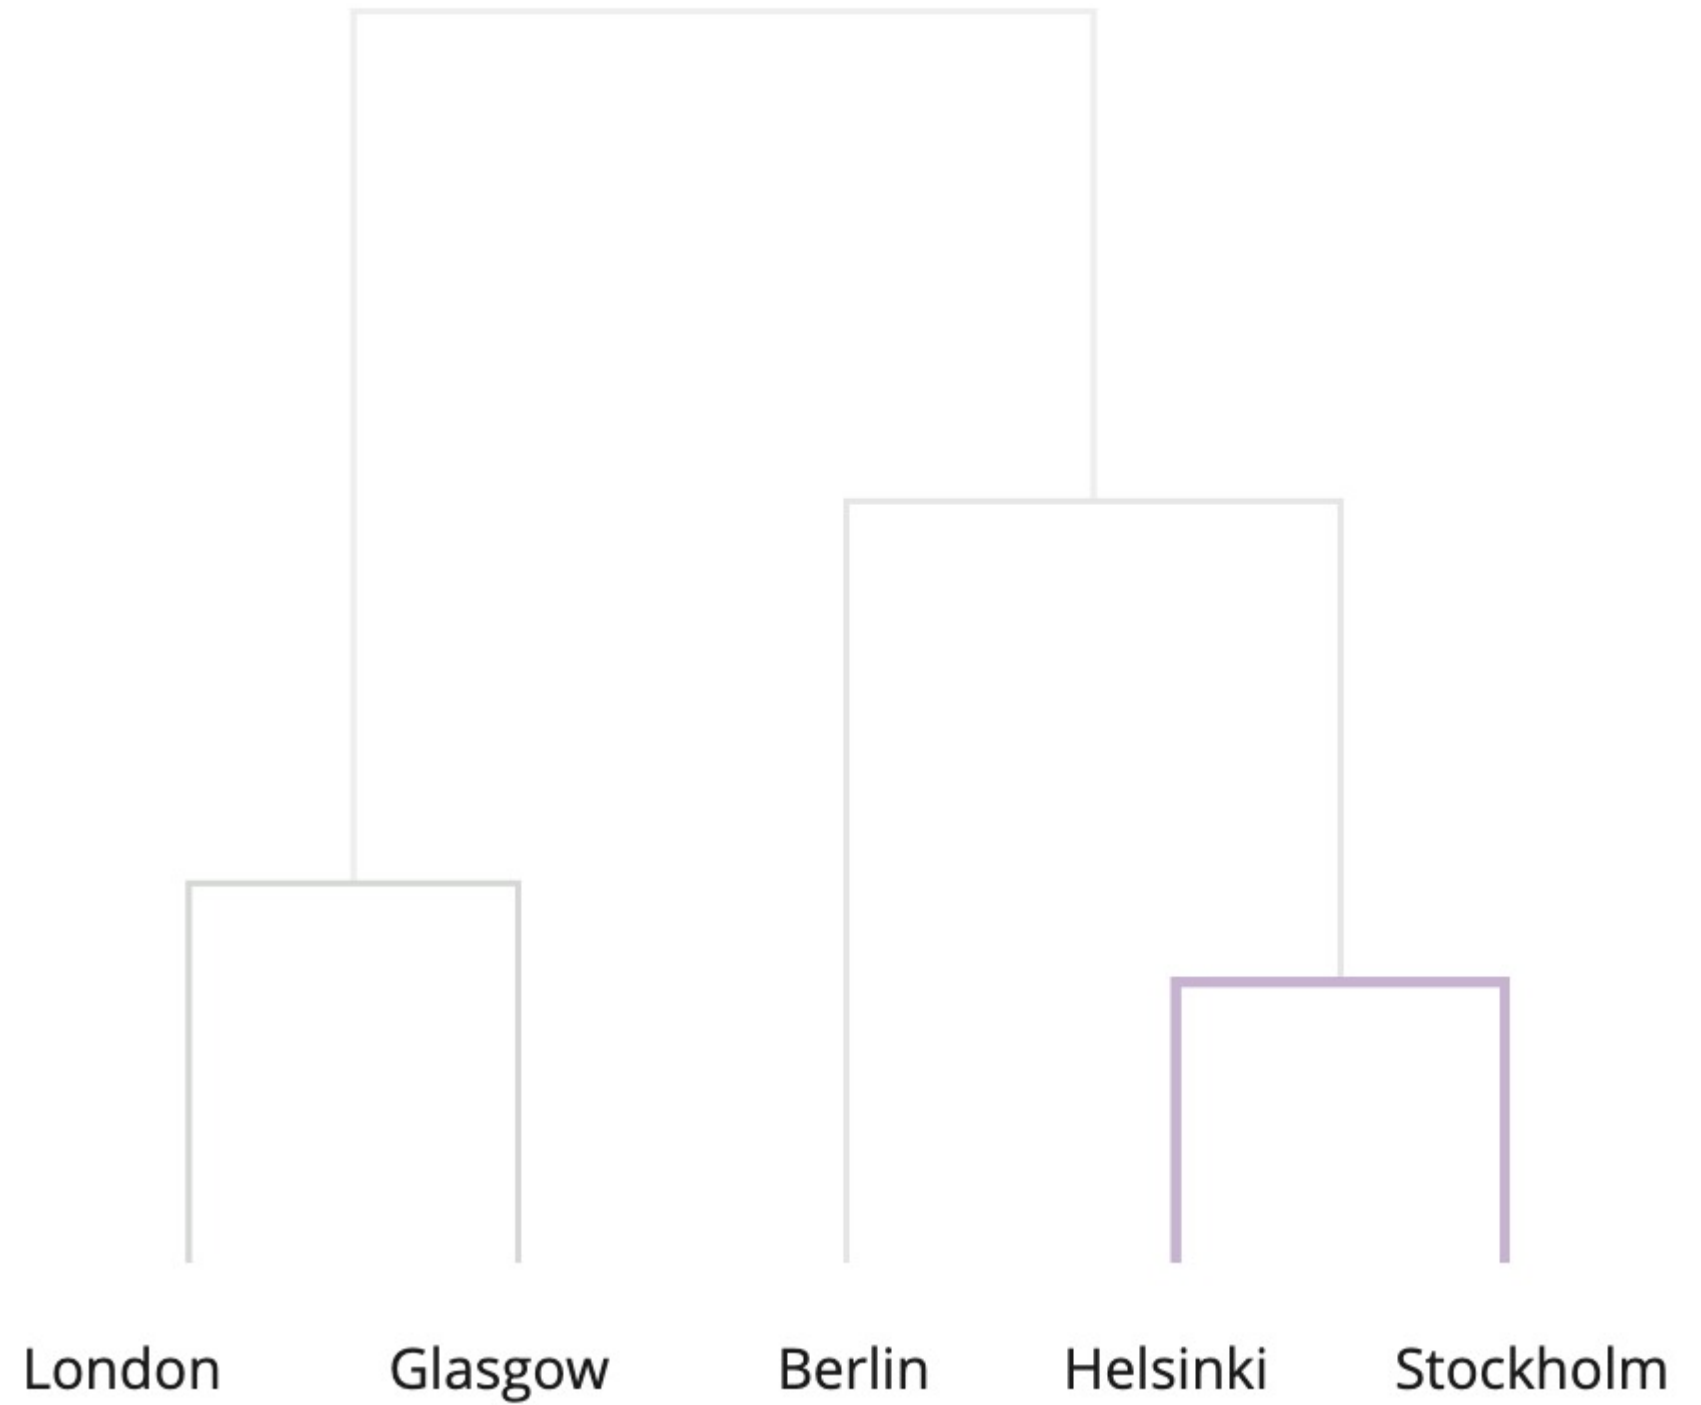

# Discrepancy Dendrogram

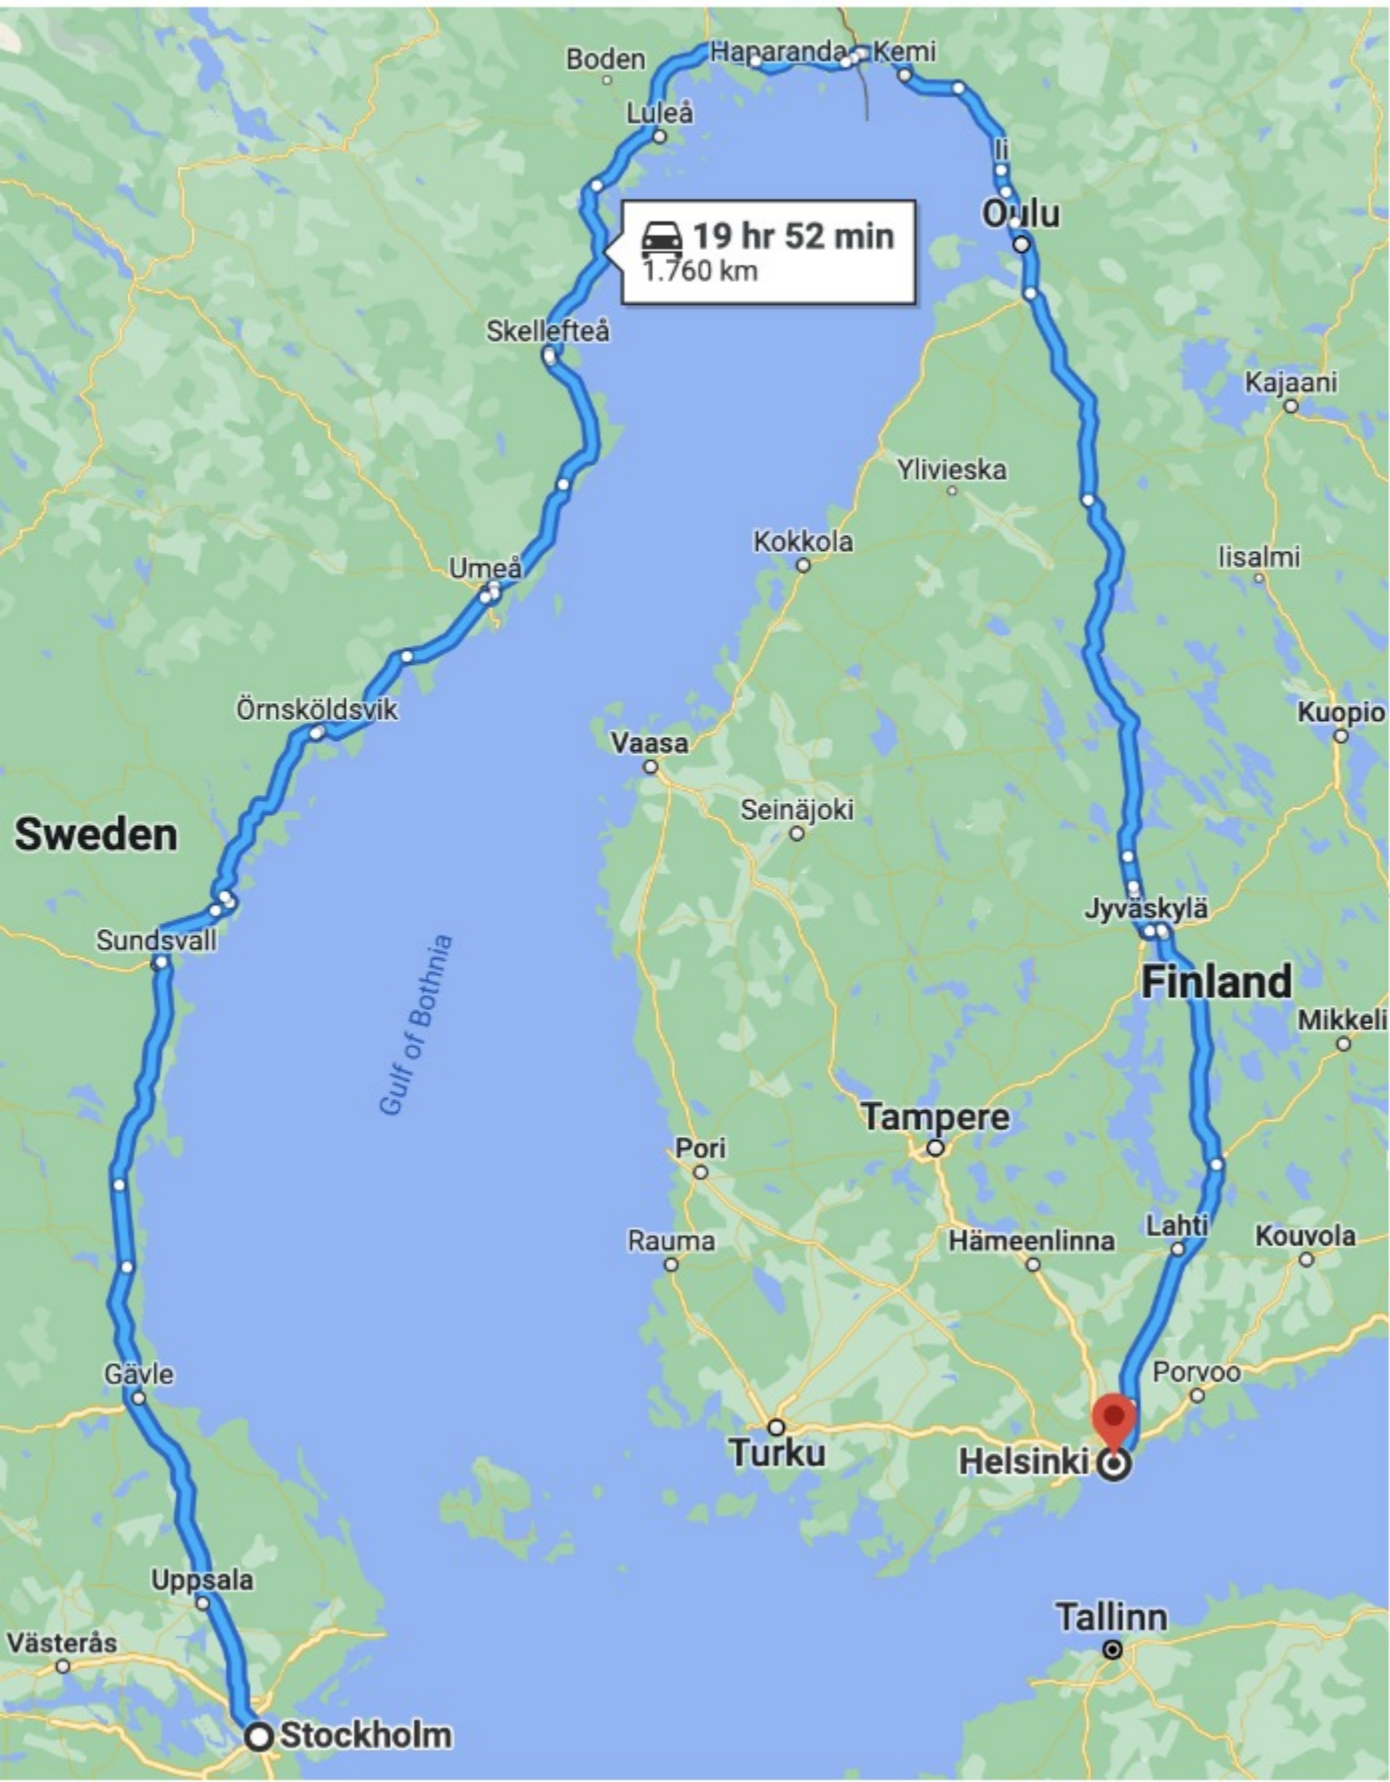

Helsinki-Stockholm:  
410 km in air  
1,760 km on ground

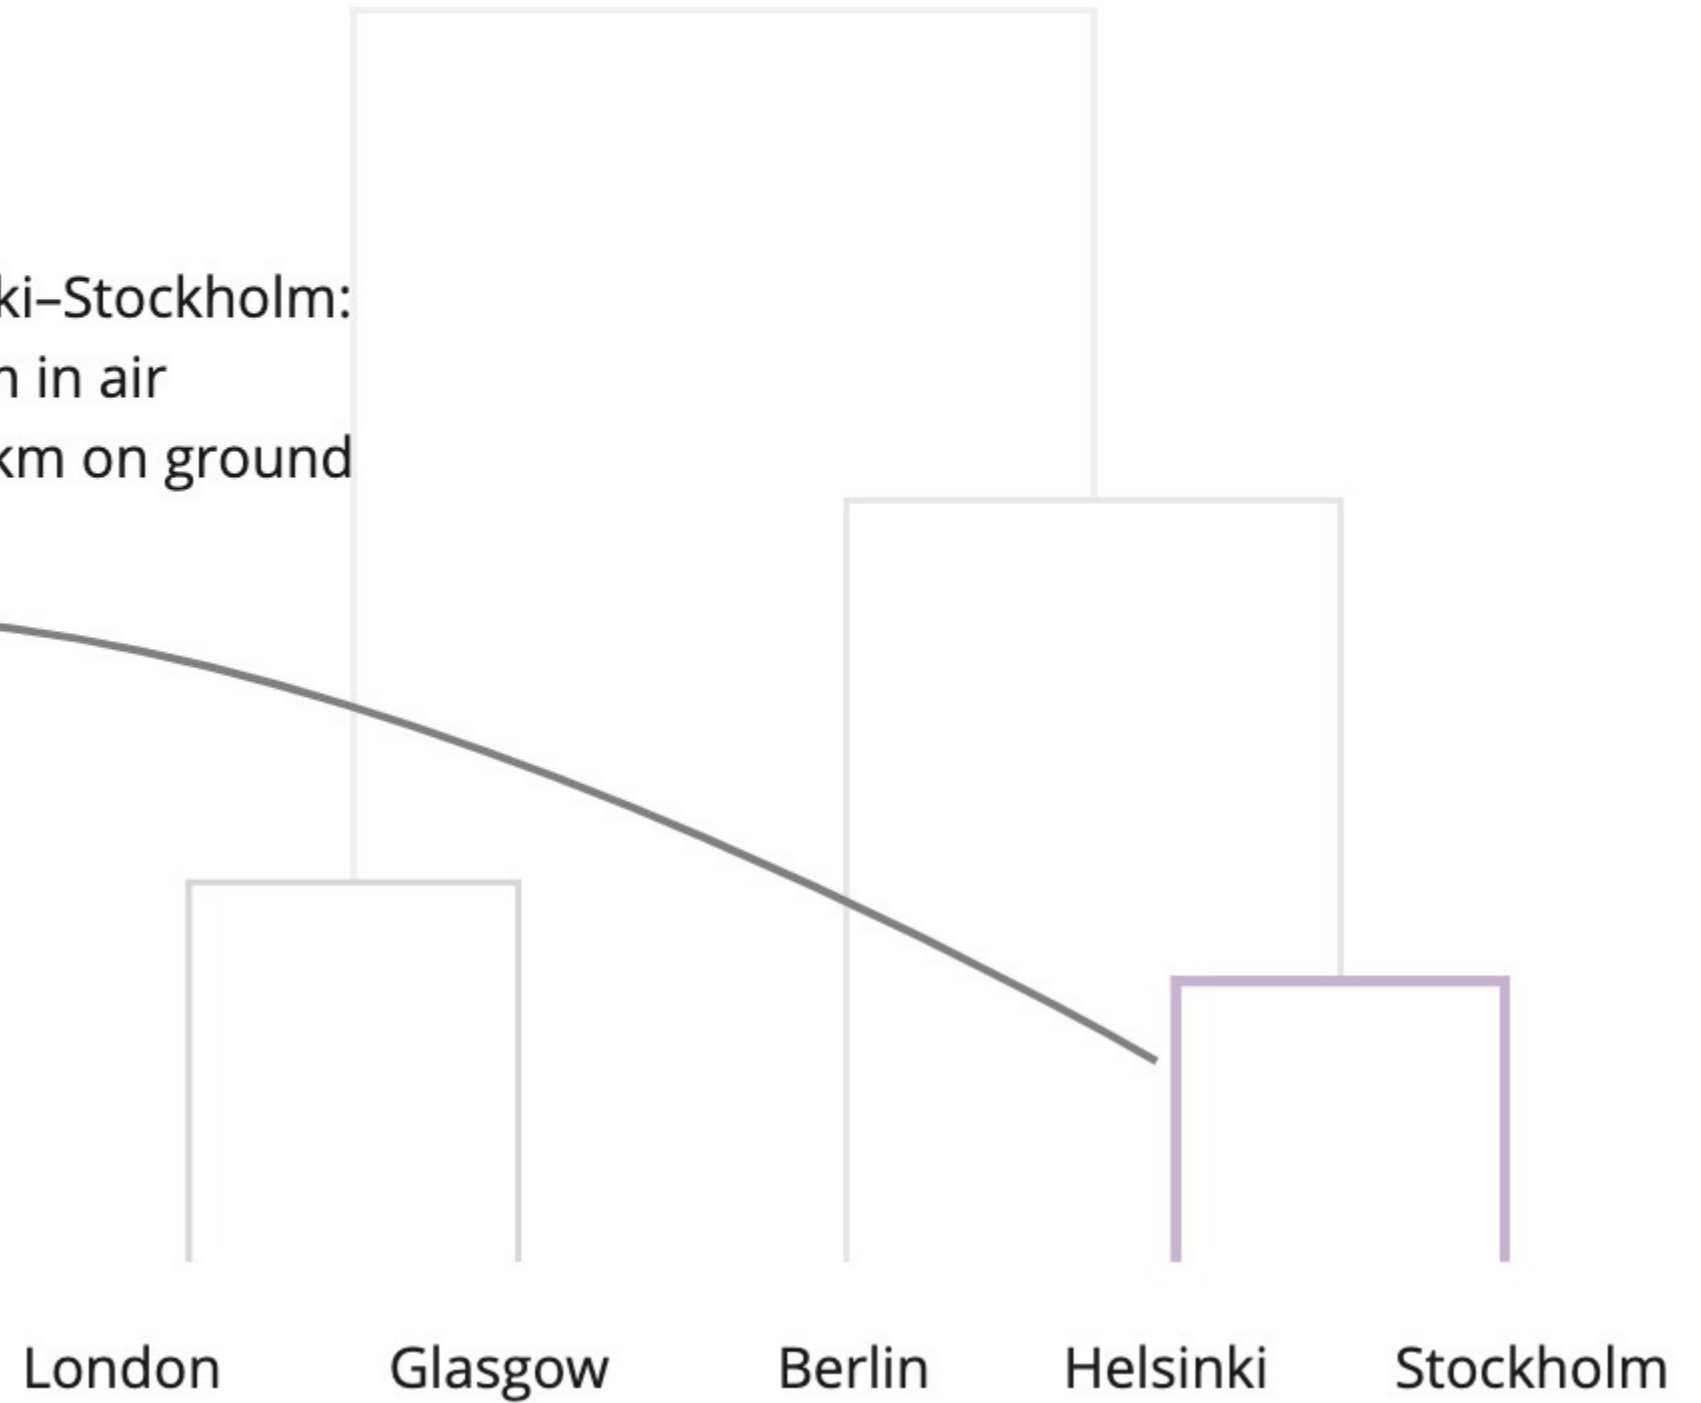

# Discrepancy Dendrogram — $X^2$

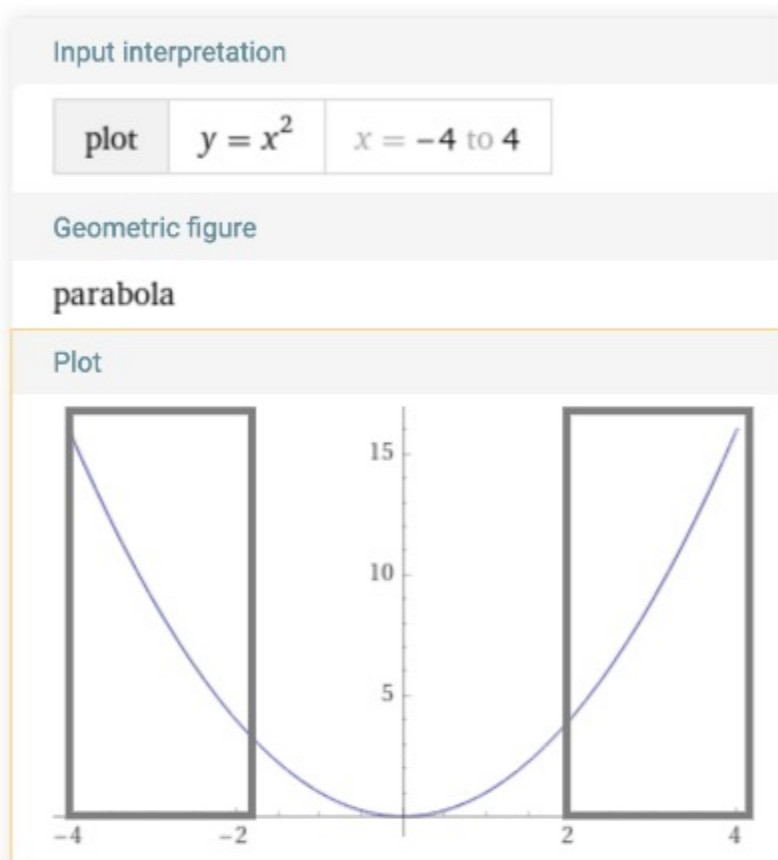

## Sensitive ranges of X

- more variation in Y

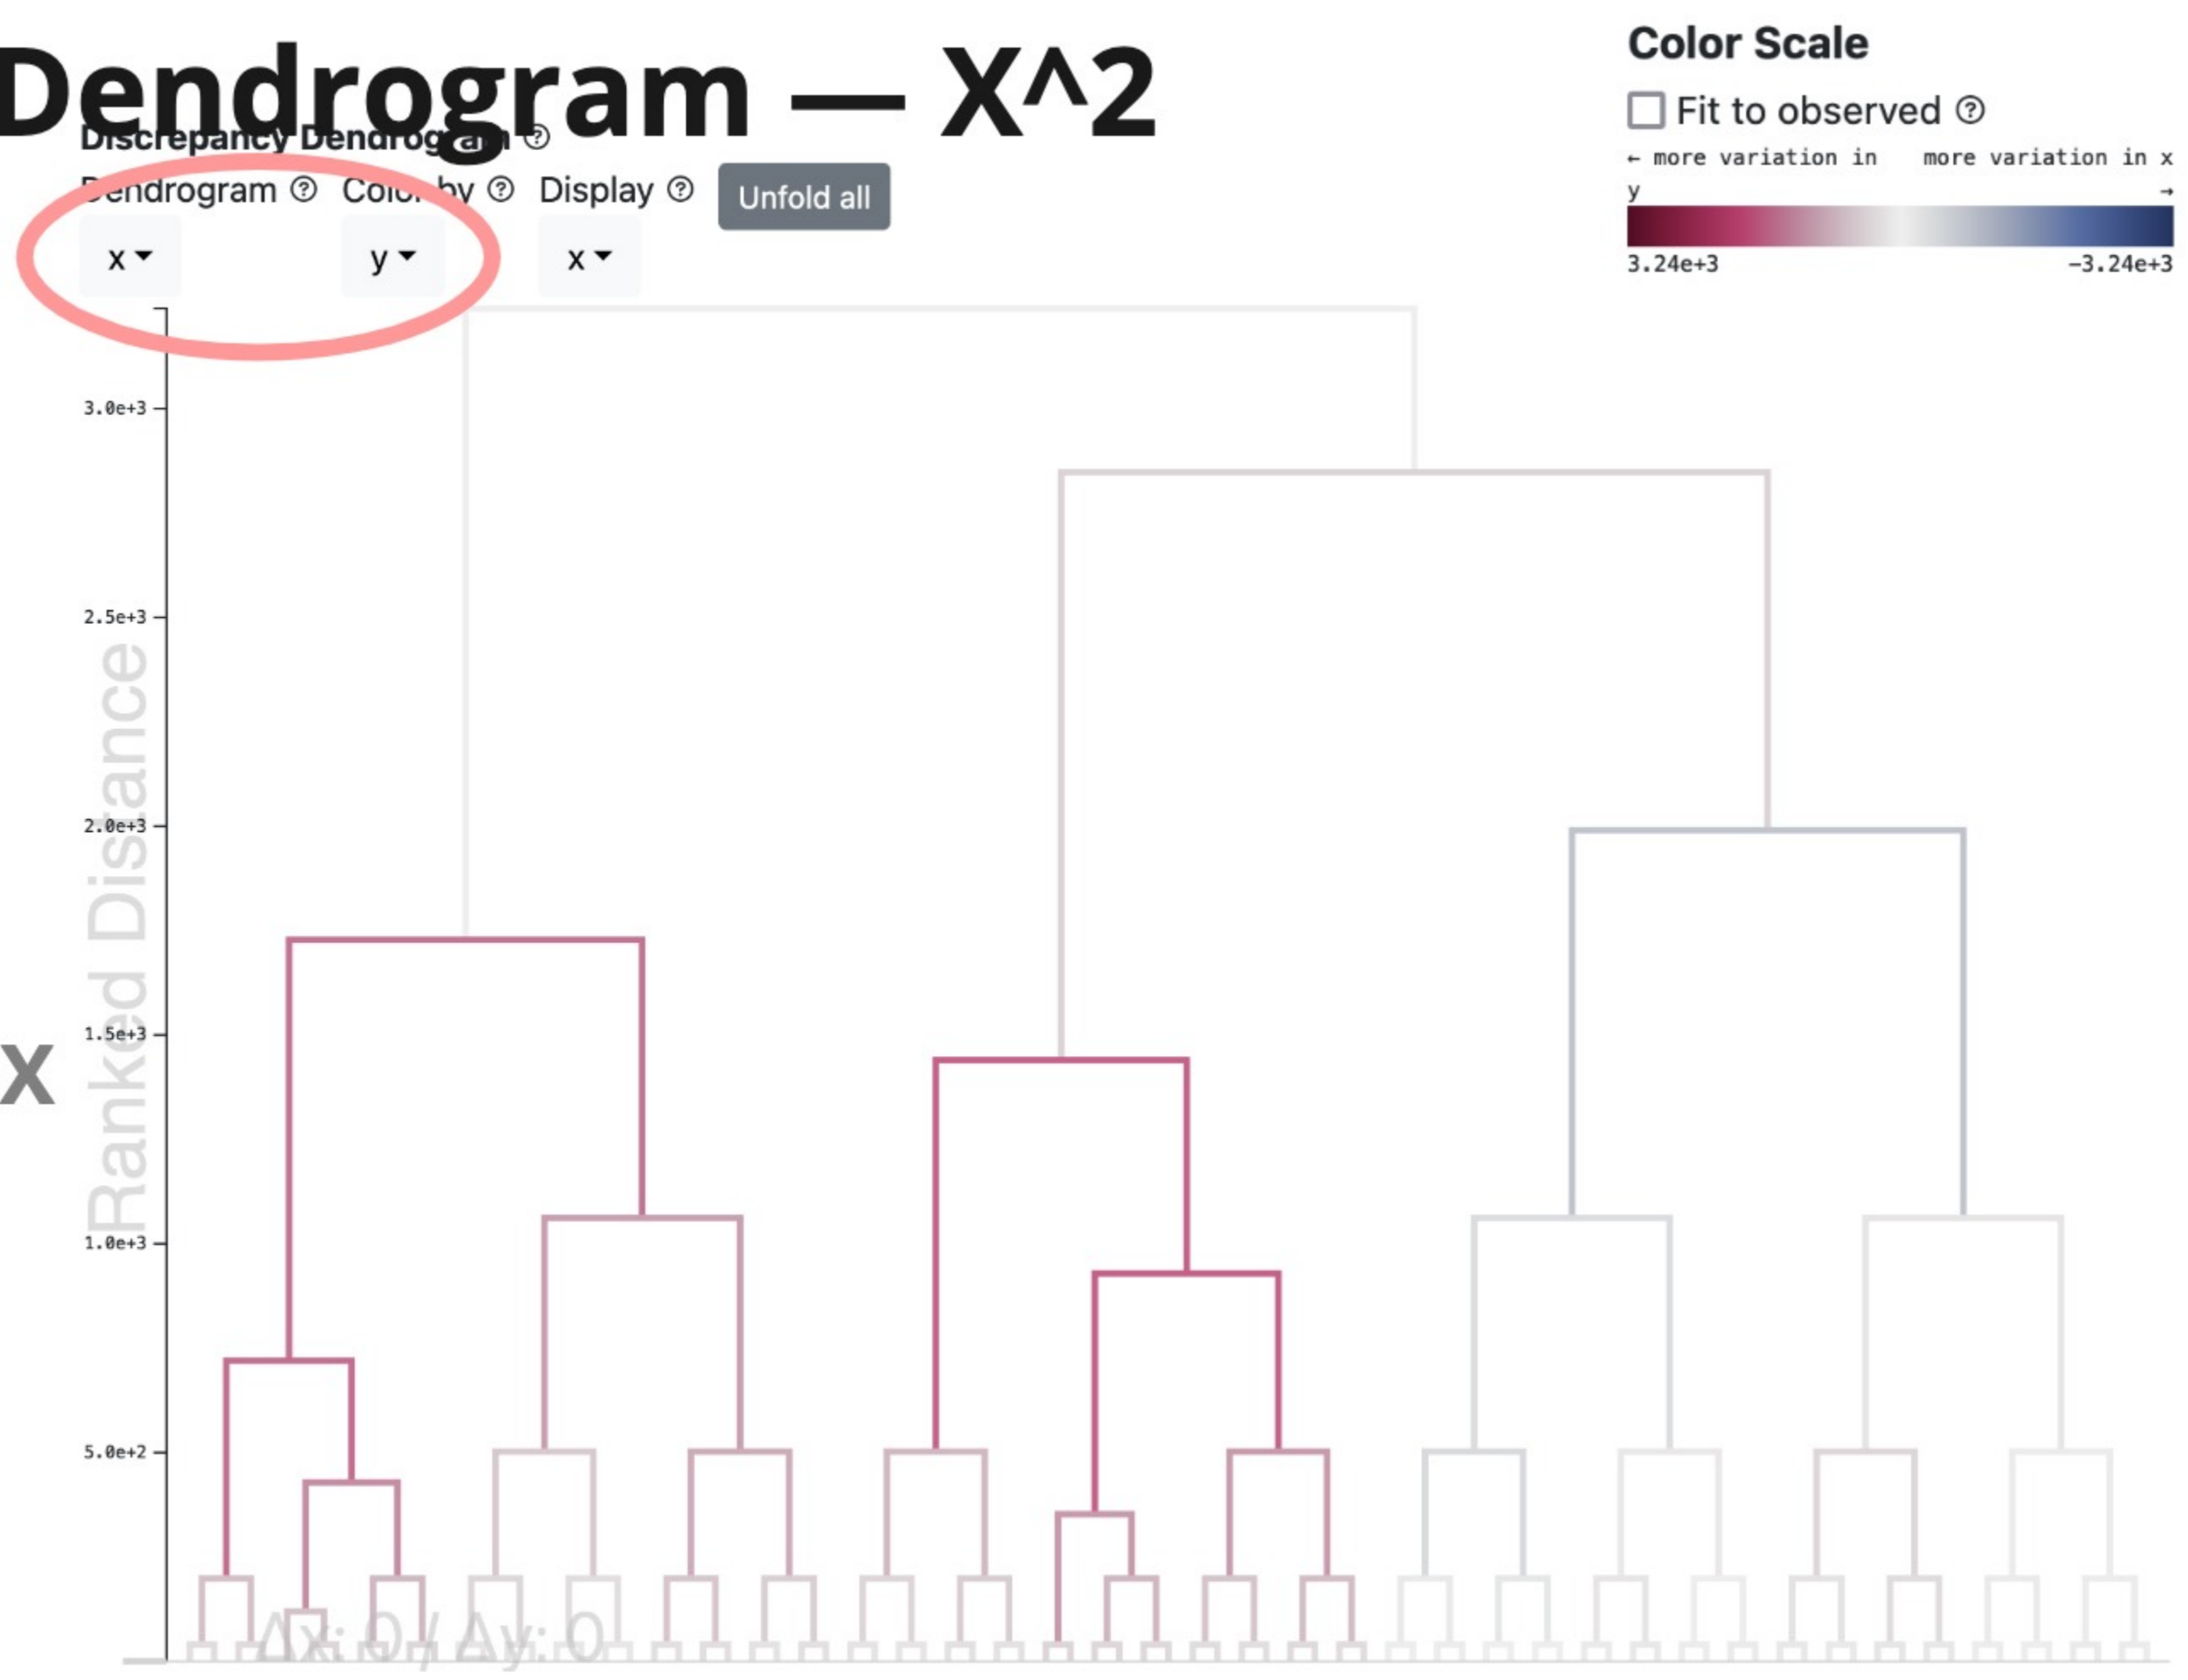

# Discrepancy Dendrogram — $X^2$

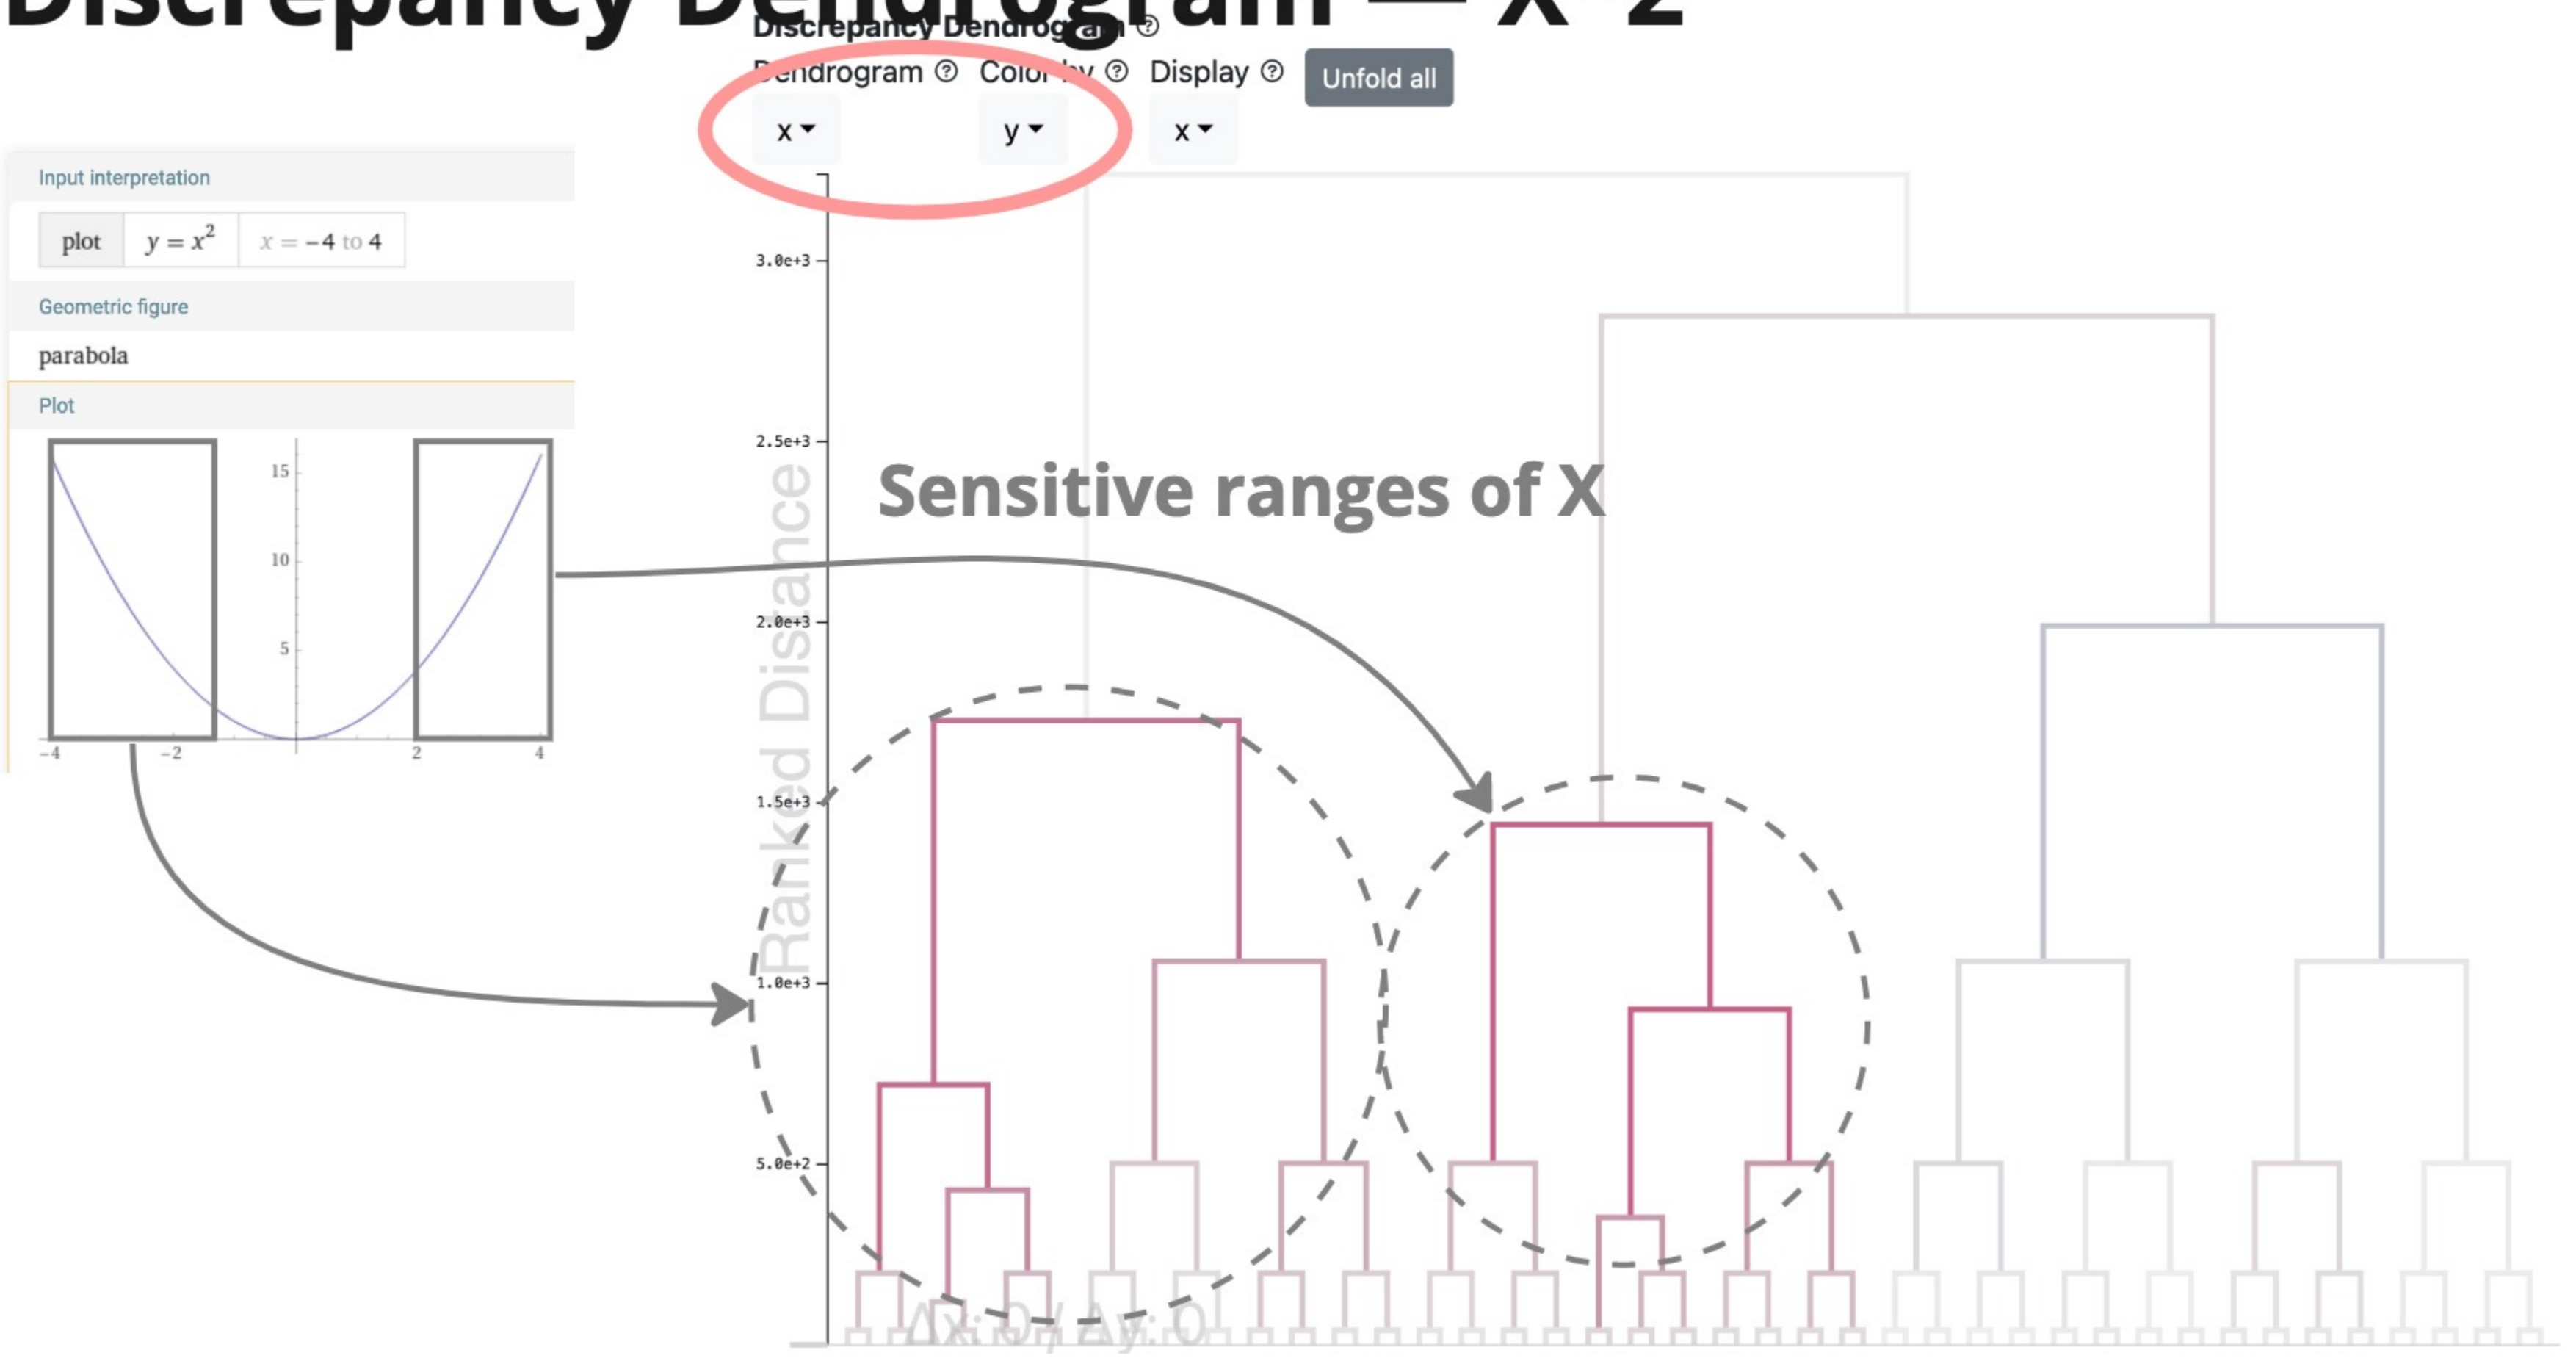

# Discrepancy Dendrogram — $X^2$

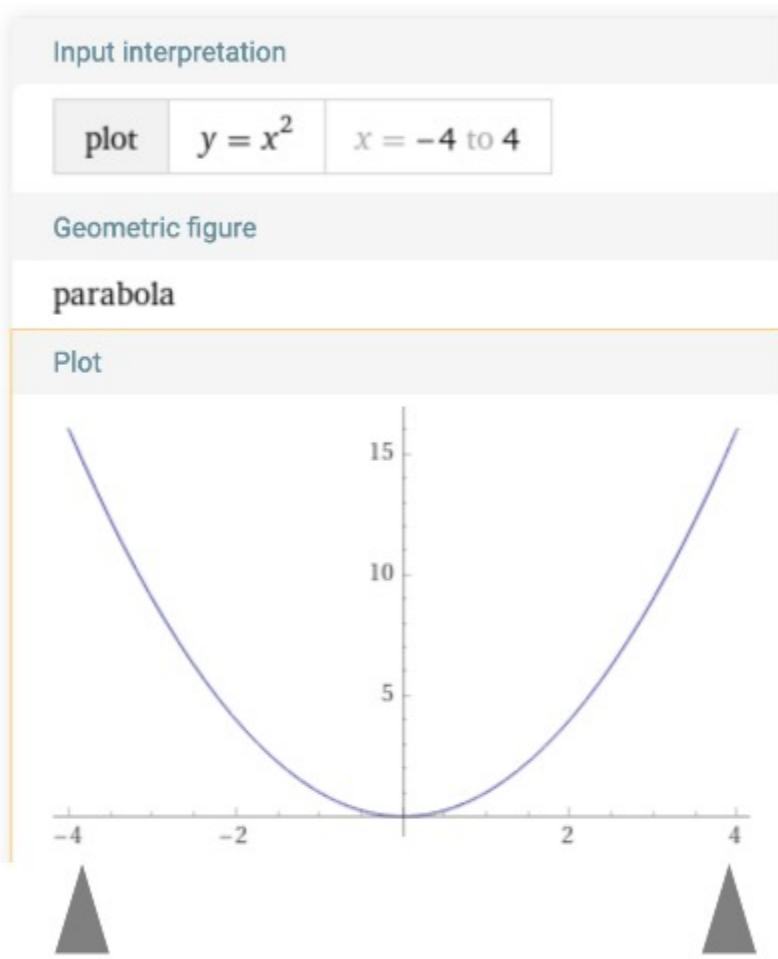

## Stable "ranges" of $X$

- more variation in  $X$

→ pairs  $(x, -x)$

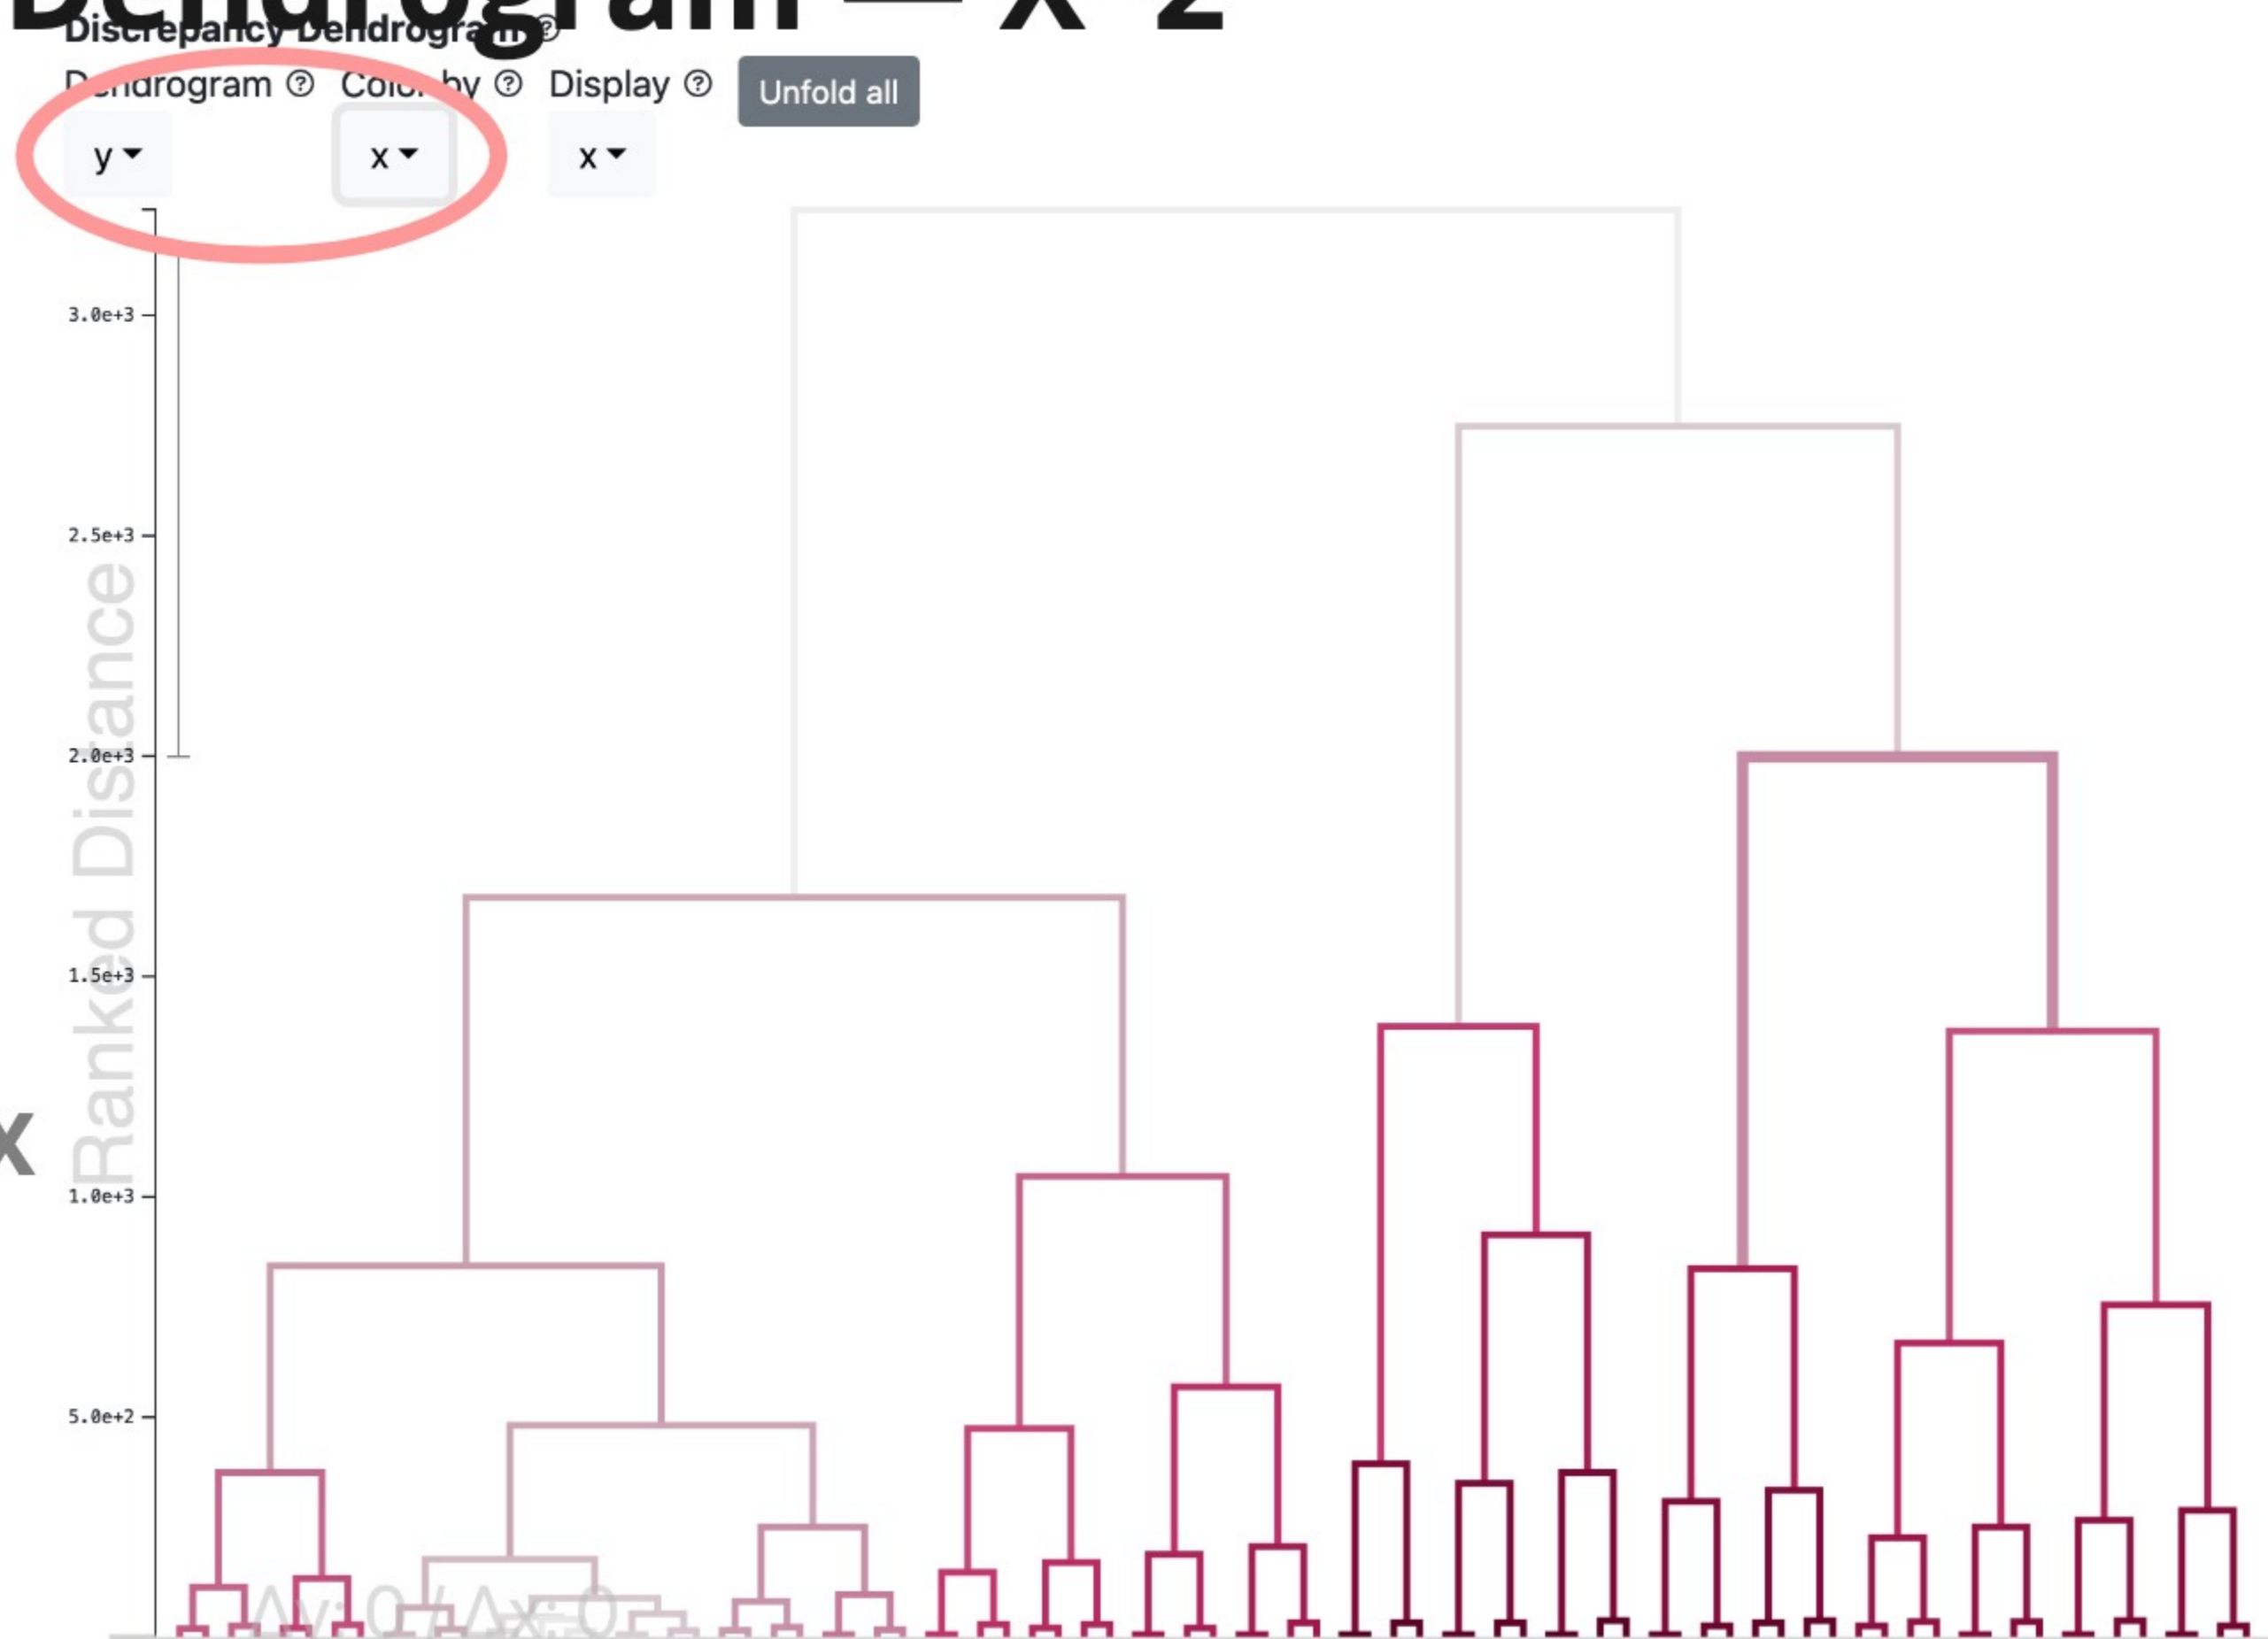

# Discrepancy Dendrogram — $X^2$

Discrepancy Dendrogram ?

Dendrogram ?

Color by ?

Display ?

Unfold all

y ▼

x ▼

x ▼

Input interpretation

plot

$$y = x^2$$

$x = -4$  to  $4$

Geometric figure

parabola

Plot

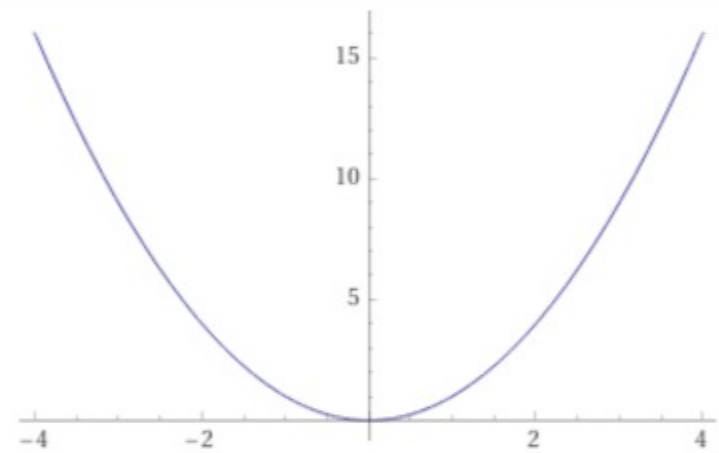

3.0e+3

2.5e+3

2.0e+3

1.5e+3

1.0e+3

5.0e+2

Ranked Distance

Stable "ranges" of  $X$

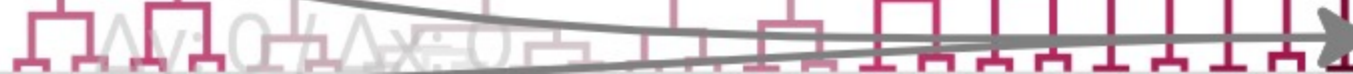

# Discrepancy Dendrogram — $X^2 * Z^2$

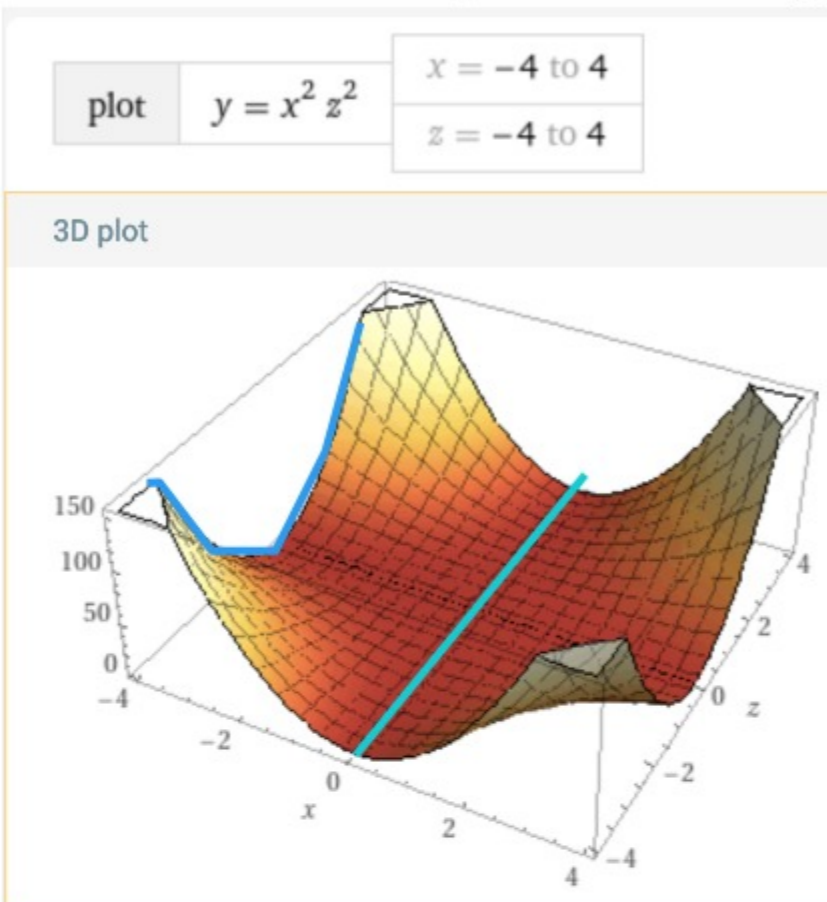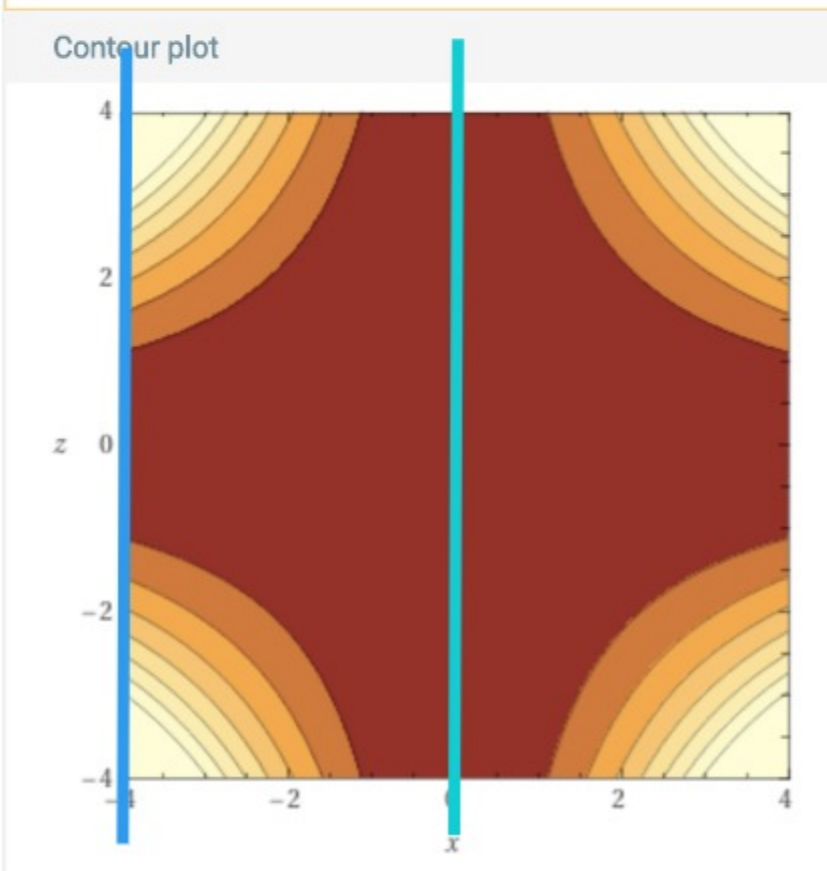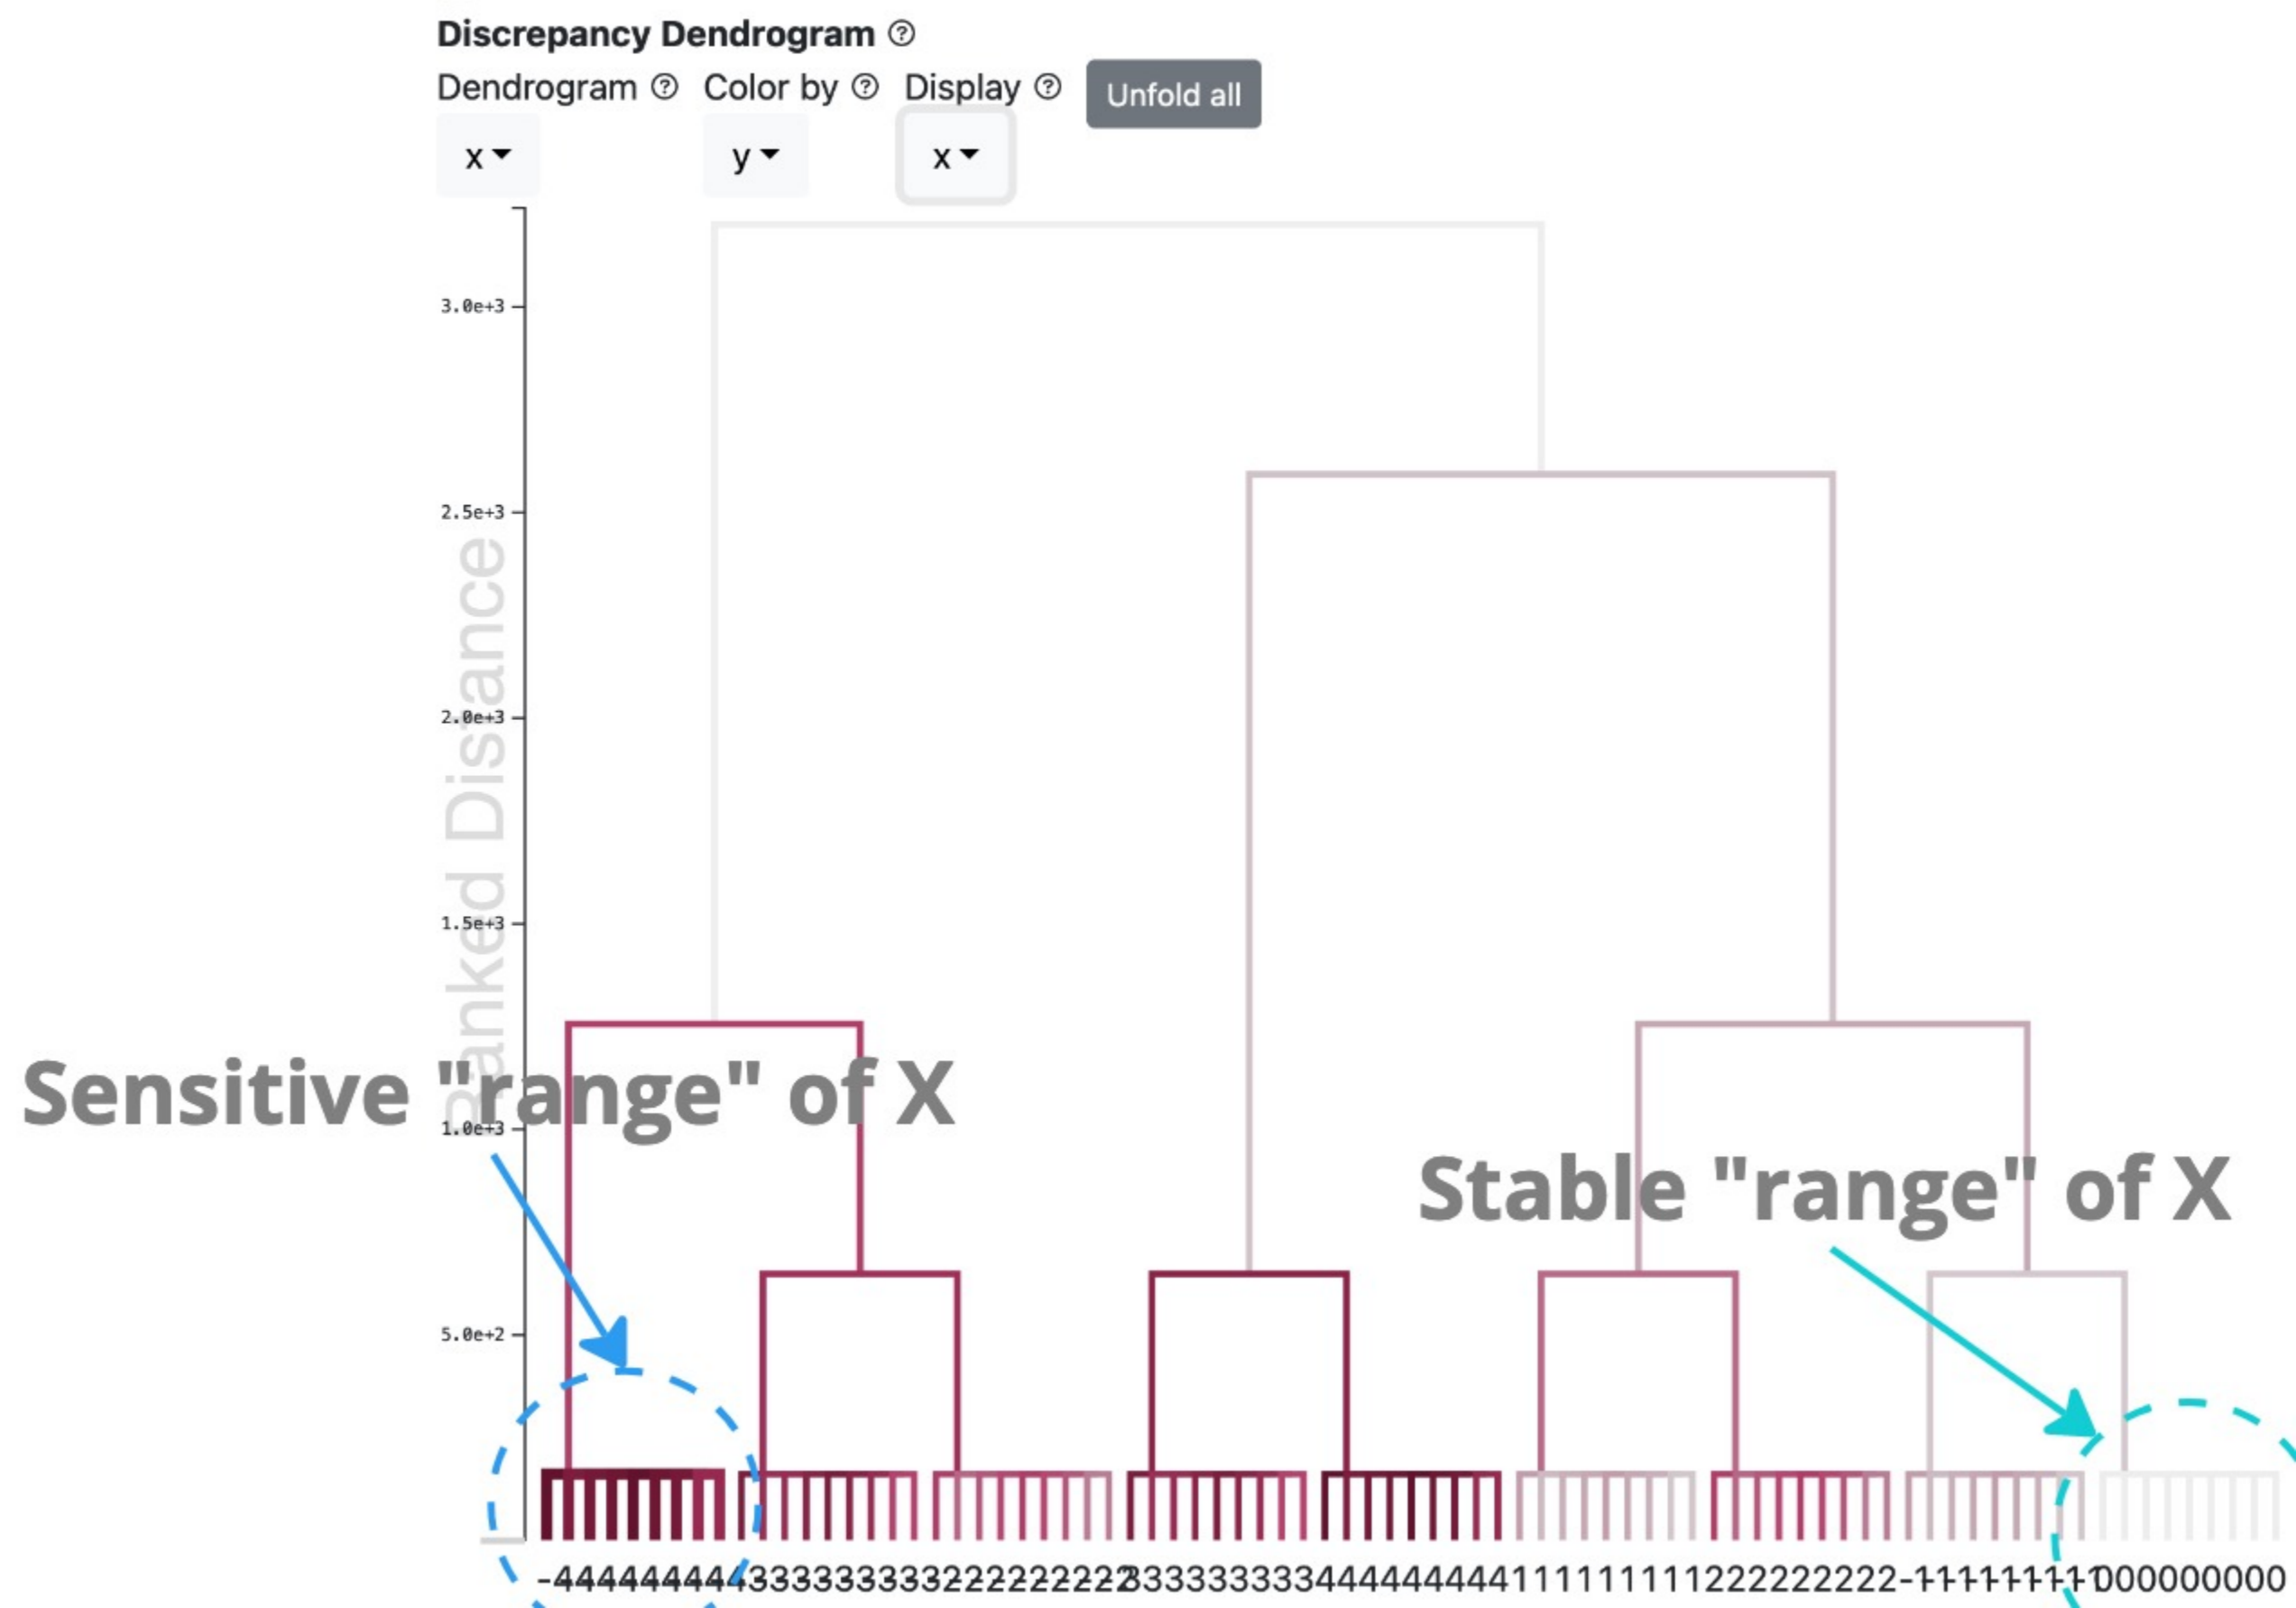

# Discrepancy Dendrogram — $X^2 * Z^2$

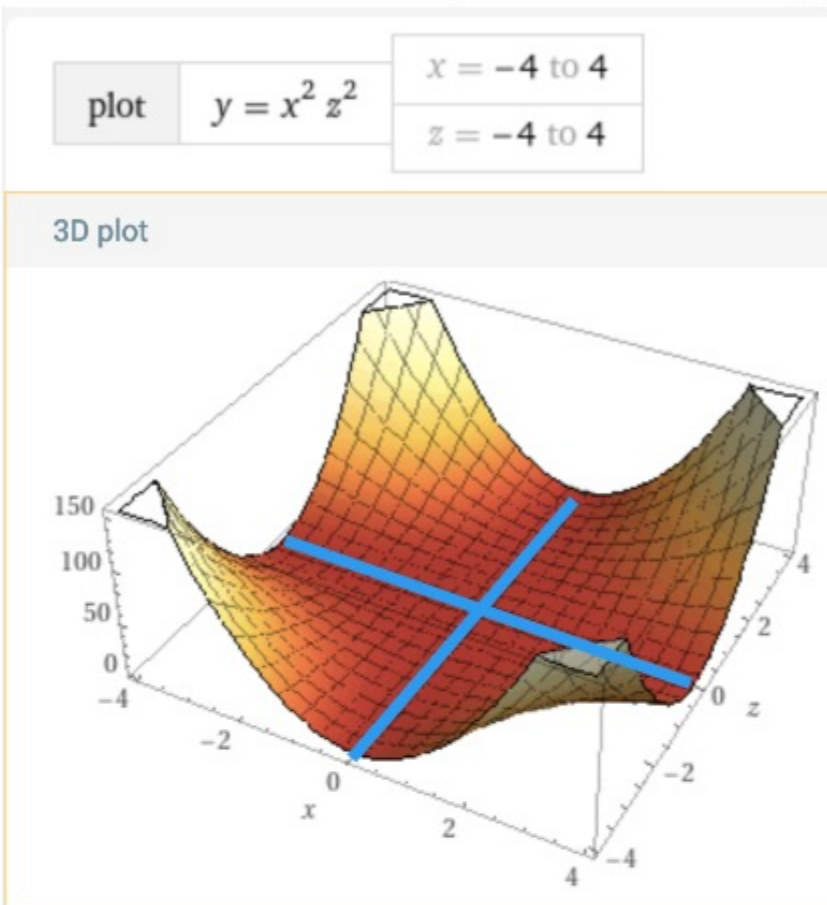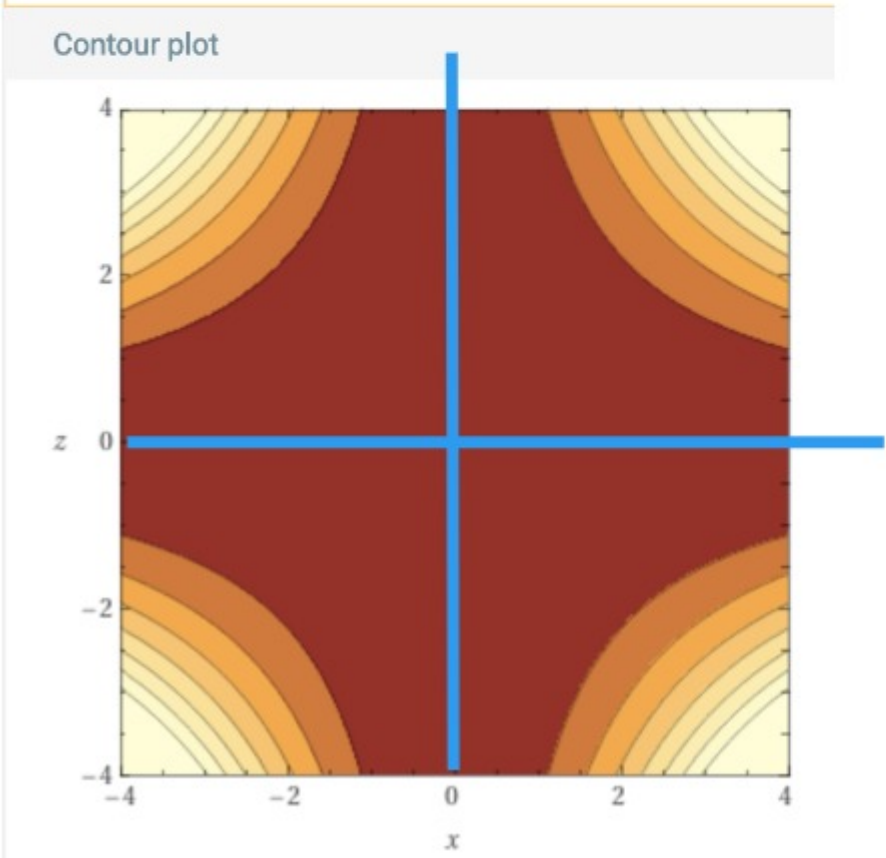

Discrepancy Dendrogram ?

Dendrogram ? Color by ? Display ? Unfold all

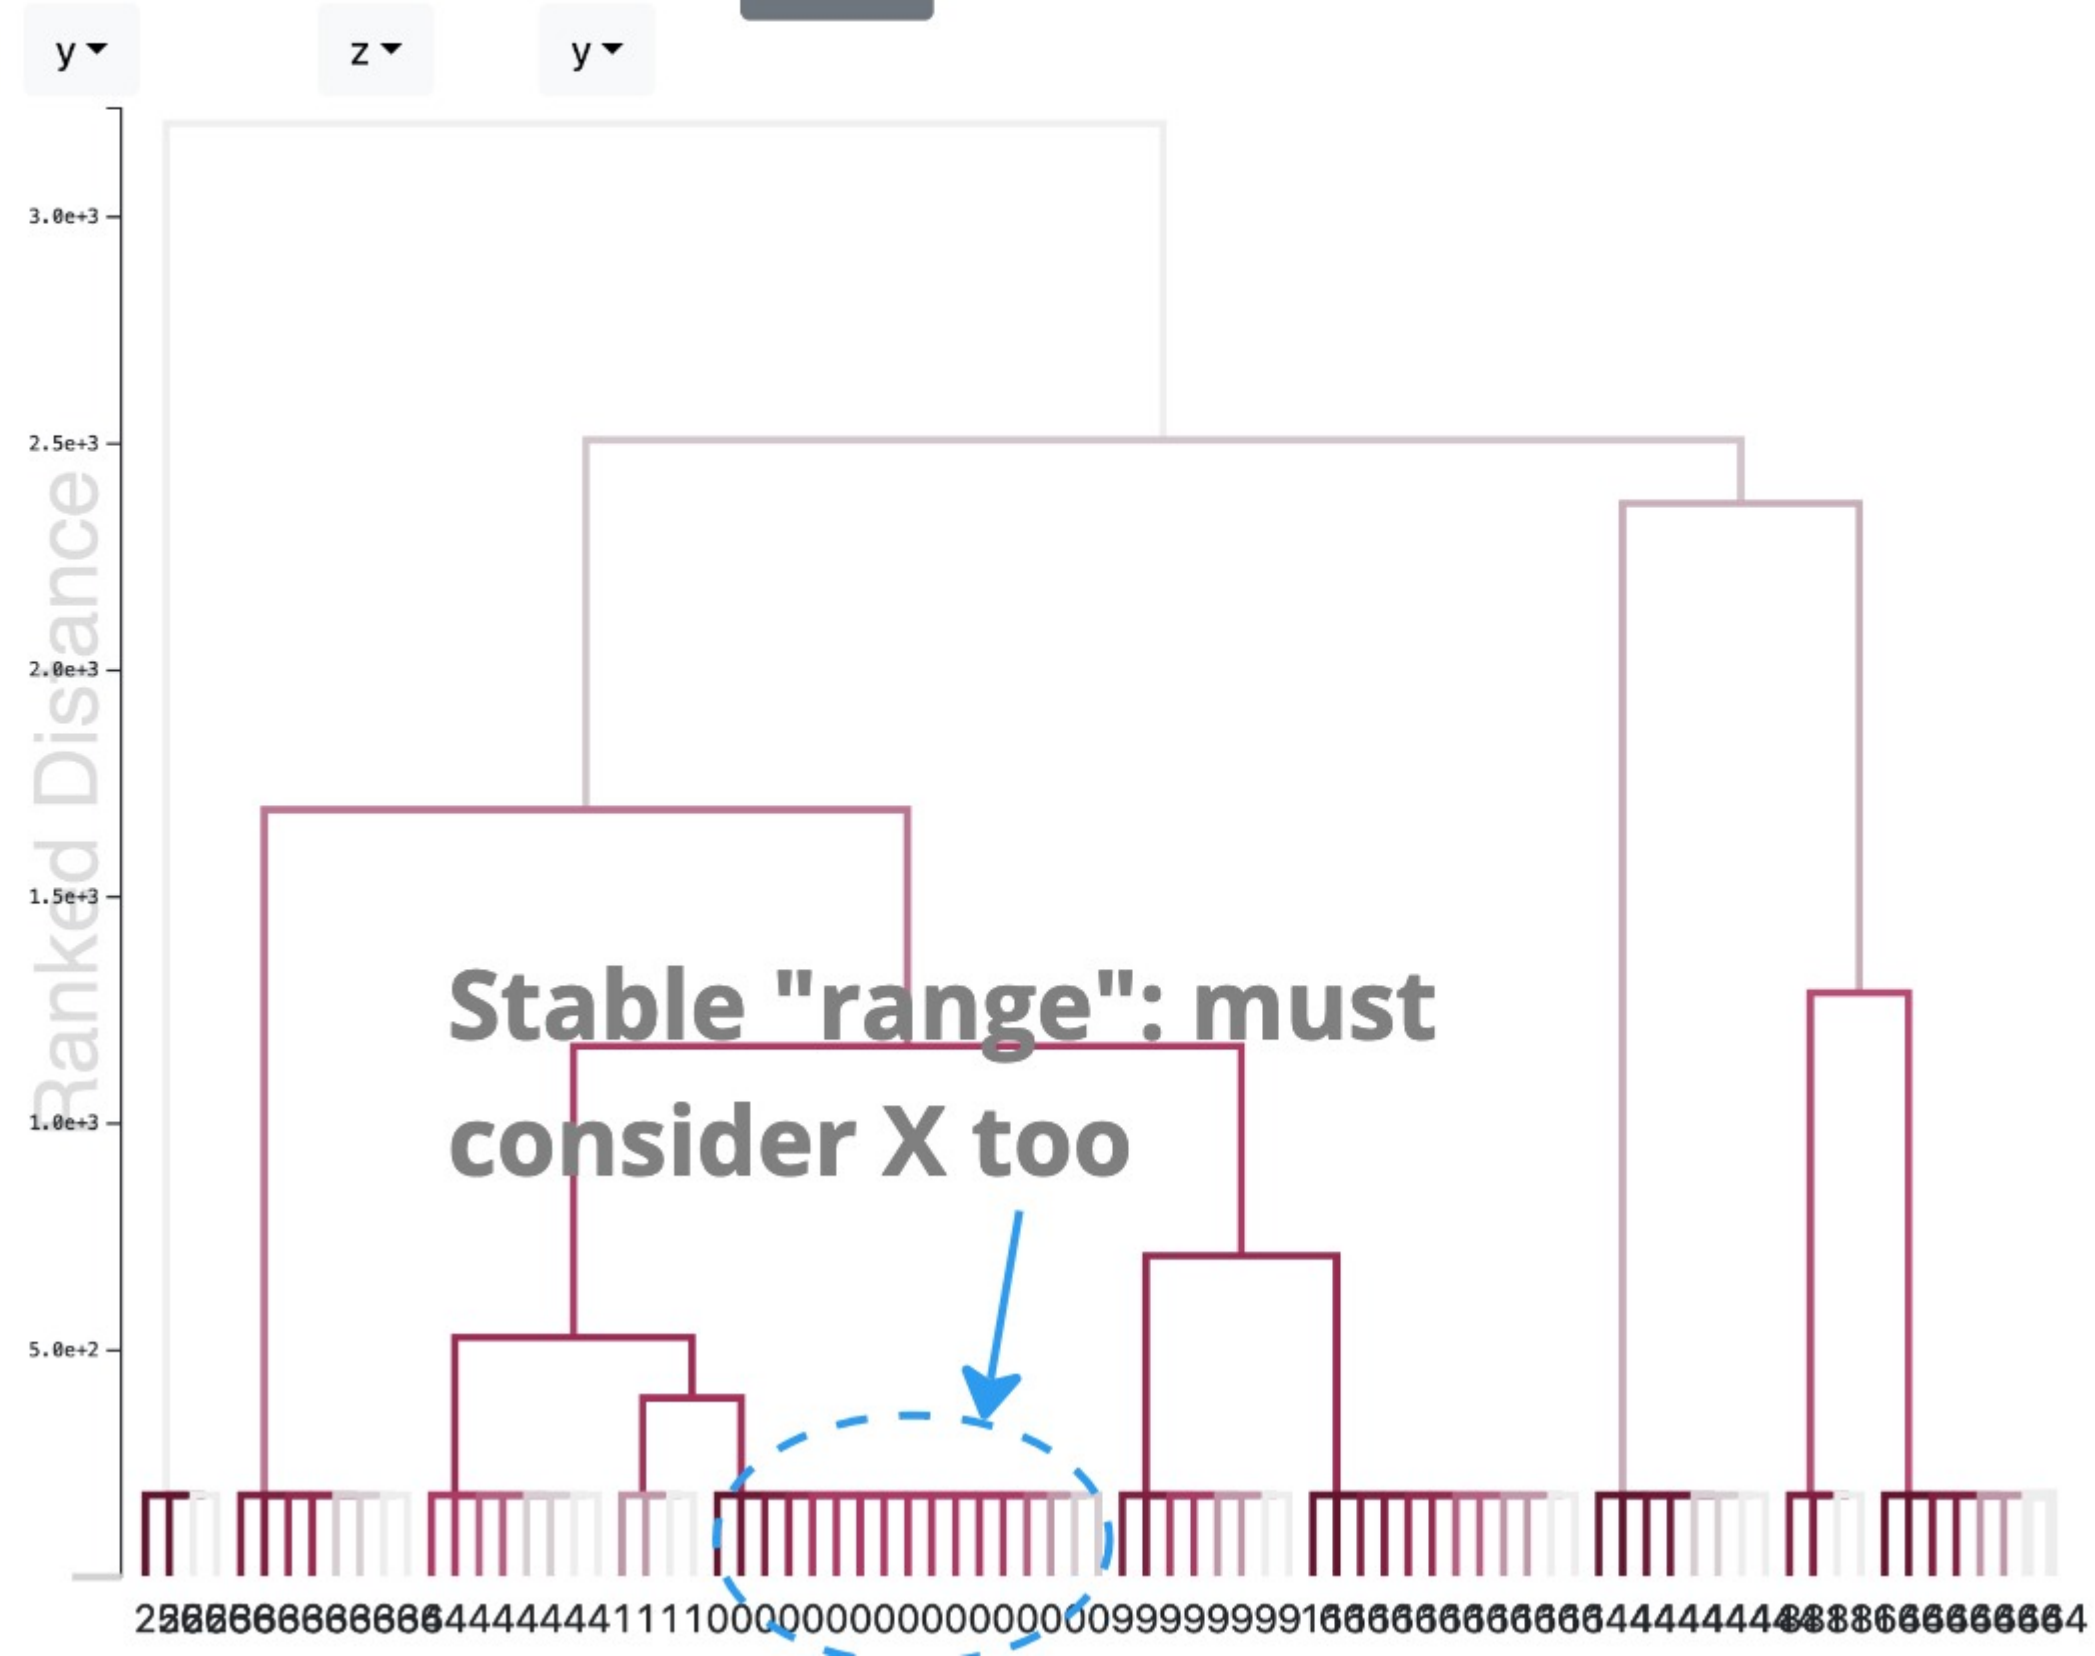

# Supporting Views

- Compare same data subsets in all similarity spaces with the Subset Sensitivity view
- Compare similarity of dissimilarity measures using Shepard matrix

Lines mark where they would be if the dendrogram was created using that dissimilarity

## Subset Sensitivity ?

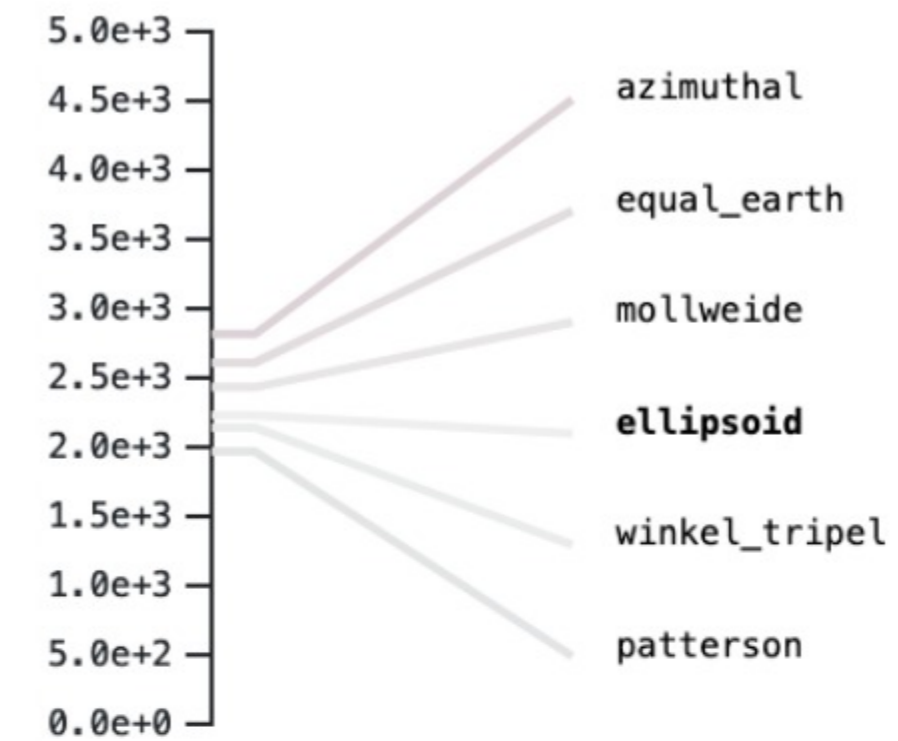

*Azimuthal equidistant*

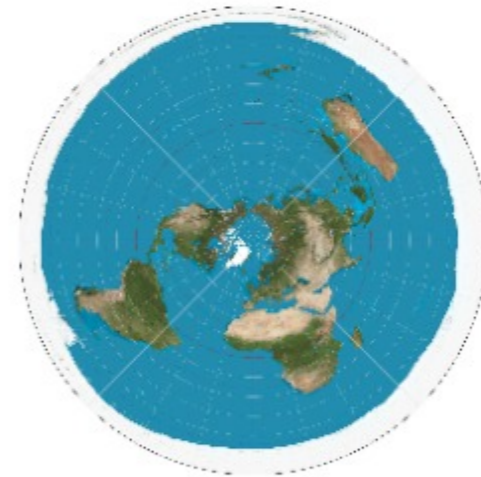

*Equal Earth*

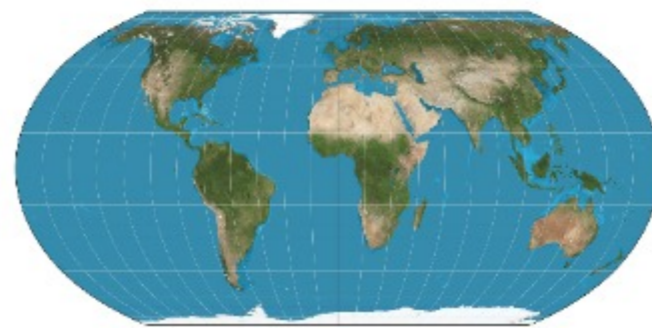

*Mollweide*

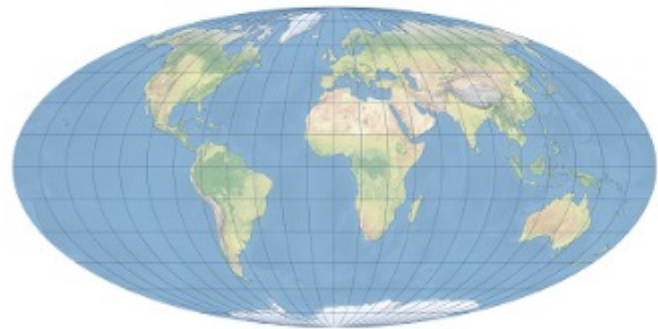

Scatterplot of pairwise distances. If scatterplot is more diagonal, the two dissimilarity measures are more alike.

## Shepard Matrix ?

**ellipsoid**

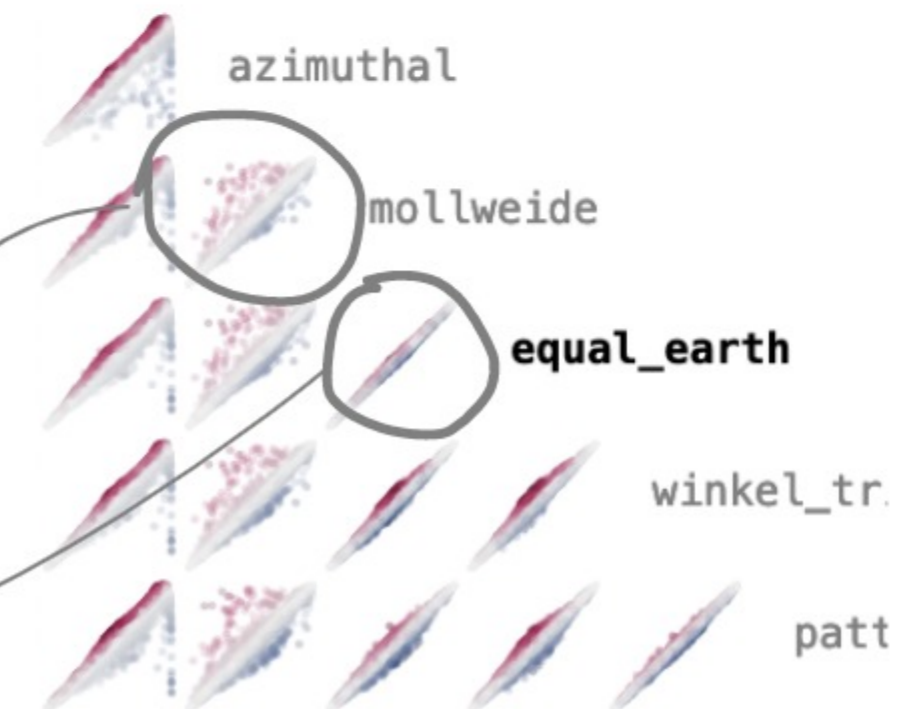

# Microclimate Dataset

- Variables
  - Input: Air temp, humidity, wind speed/dir
  - Output: Air/surface temp, humidity, wind speed
- 12 parameter/output tuples
- Dissimilarity measure  $d(., .)$ : Euclidean distance

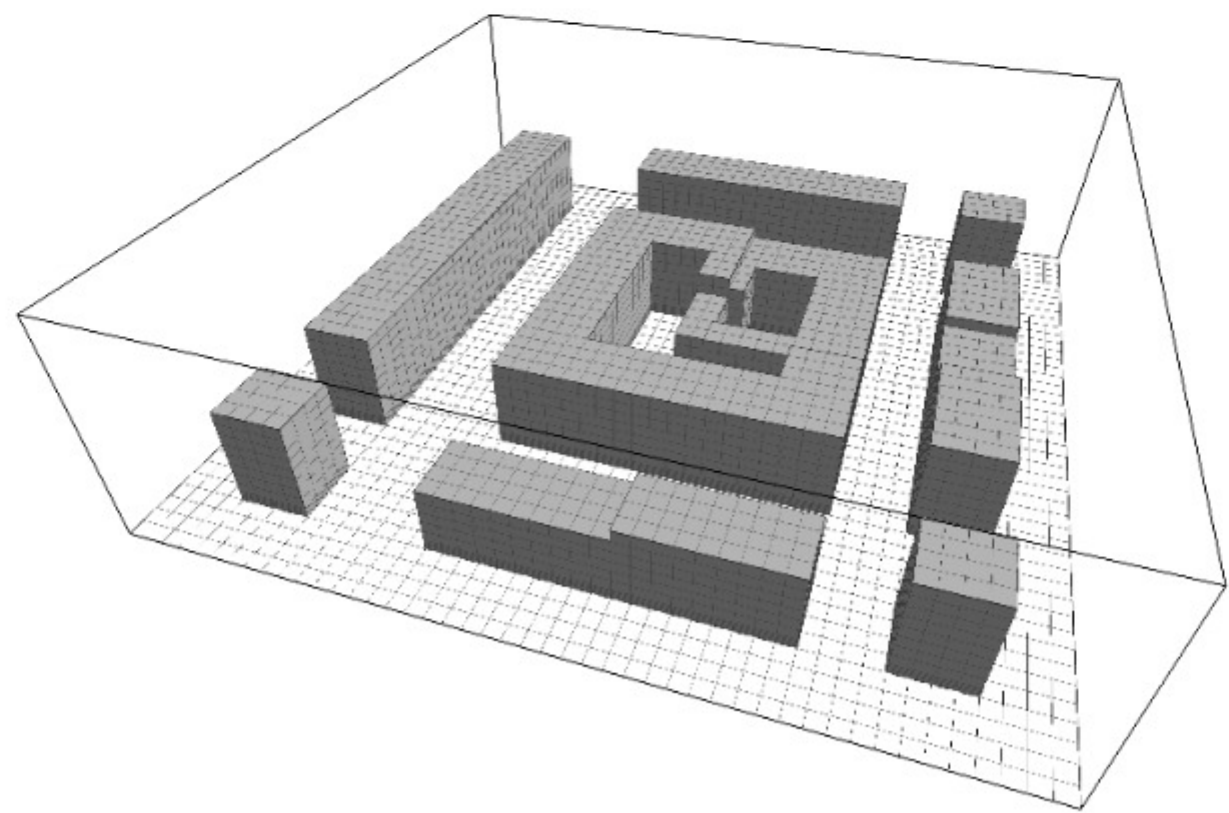

# Microclimate Dataset: Visualizations

- Output (on grid): Heatmaps with different hue per type (temp = orange, wind = blue, humidity = green)
- Input (time series): Line chart
- Input (vector): Arrow

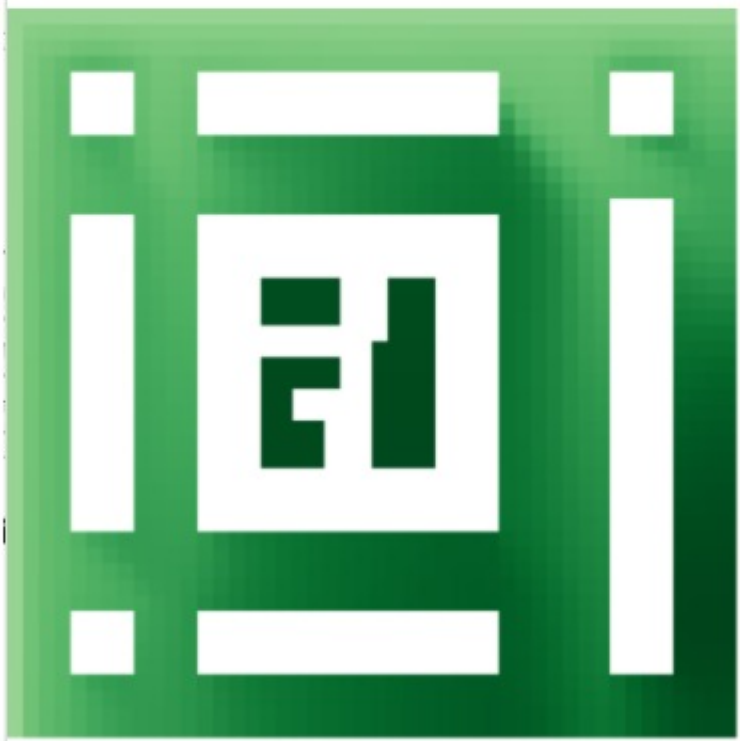

humidity output

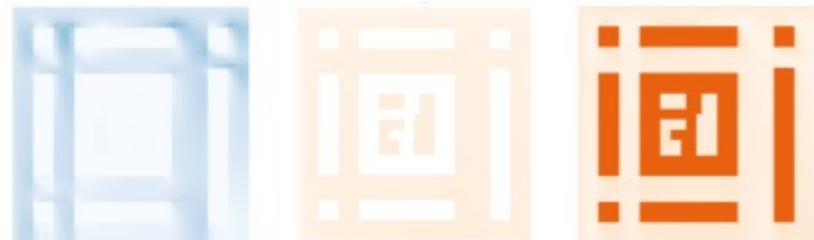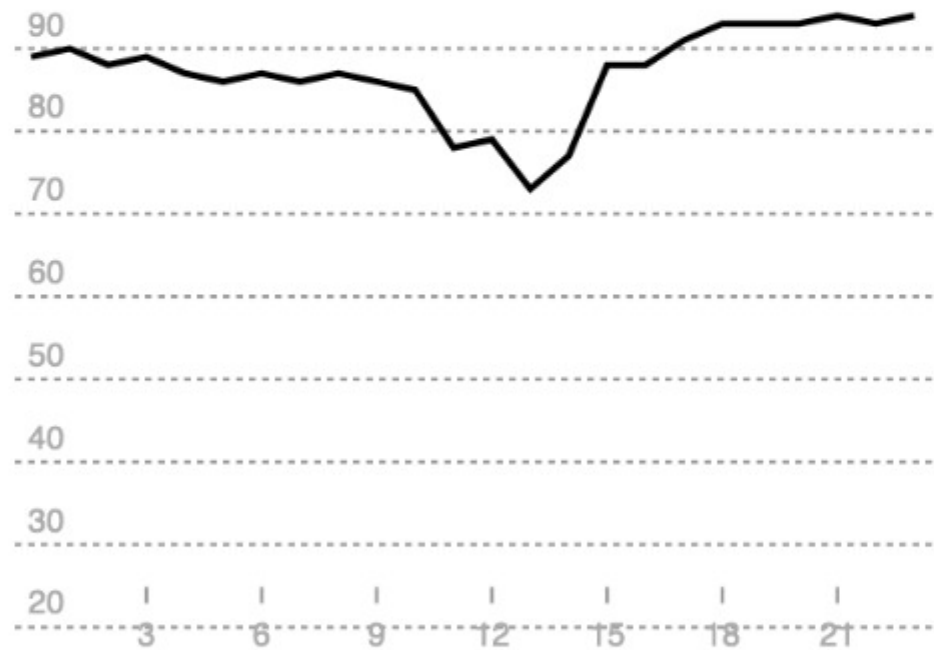

humidity input

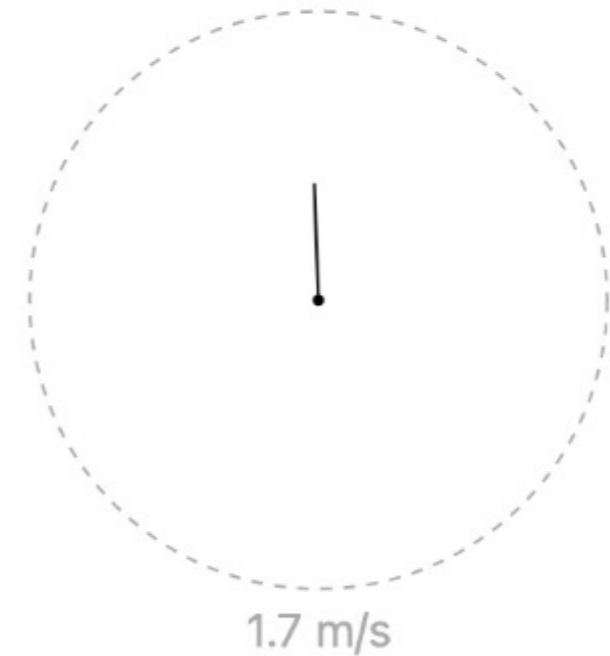

wind input

# Demo time

[link](#)

# SNSS Colorado Dataset

- Variables: unmixing matrix  $\mathbf{w}$ , kernels  $\mathbf{k}$ , regionalizations  $\mathbf{r}$
- 6 kernels x 8 regionalizations = 48 combinations
- Dissimilarity measures  $d(., .)$ :
  - $\mathbf{w}$ : MD Index
  - $\mathbf{r}$ : Percentage of location pairs that have unequal relation (in same region or not)
  - $\mathbf{k}$ : Norm of difference of the spatial kernel matrices

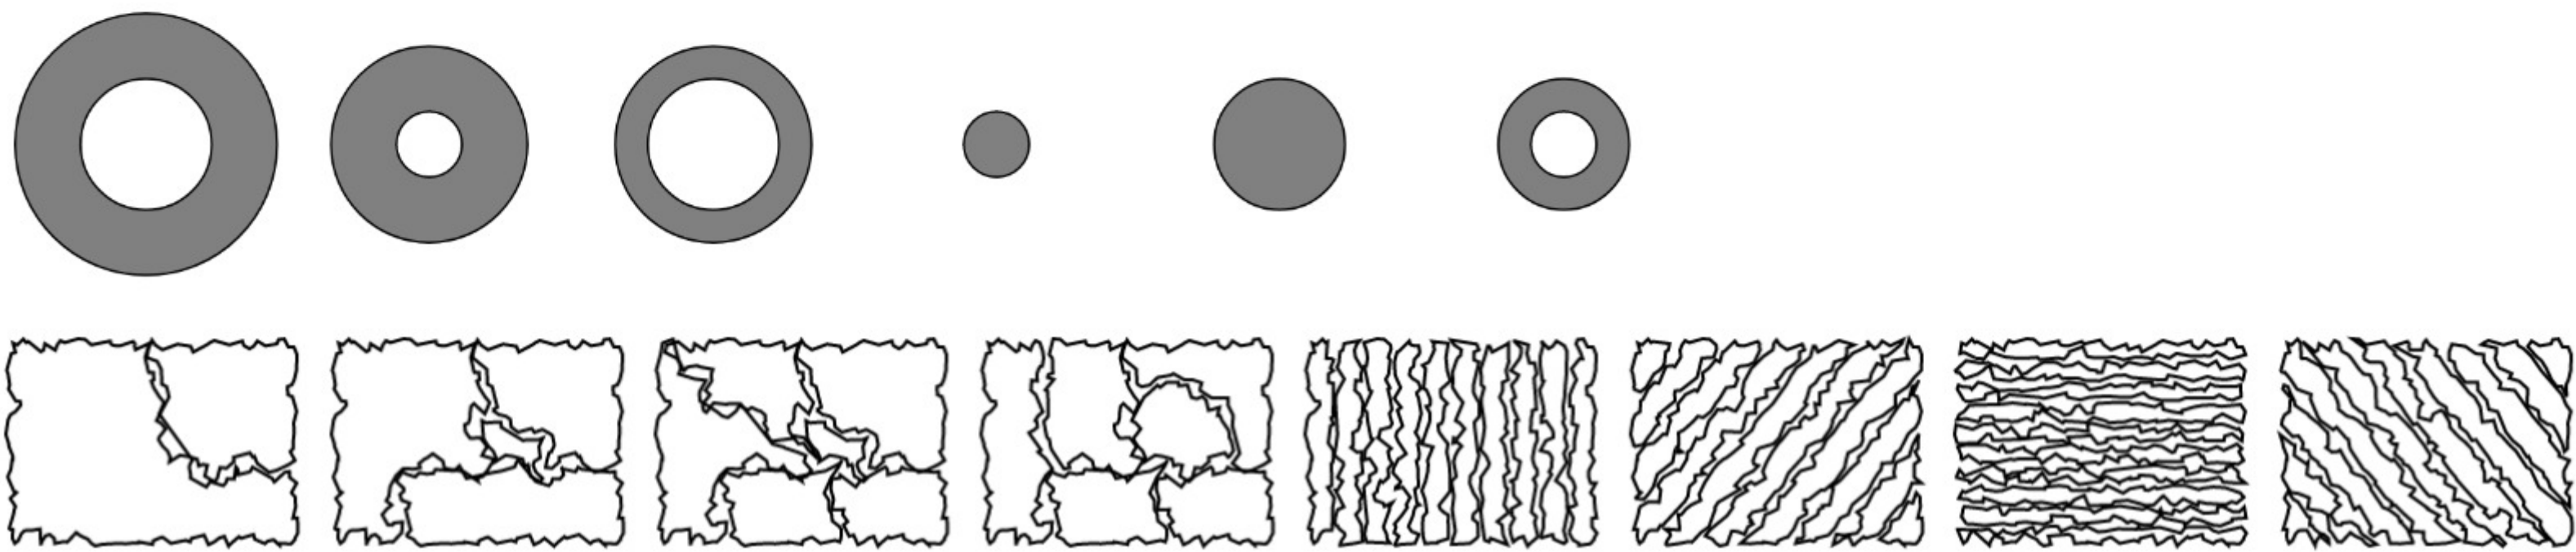

# SNSS Colorado Dataset

- Output visualization:

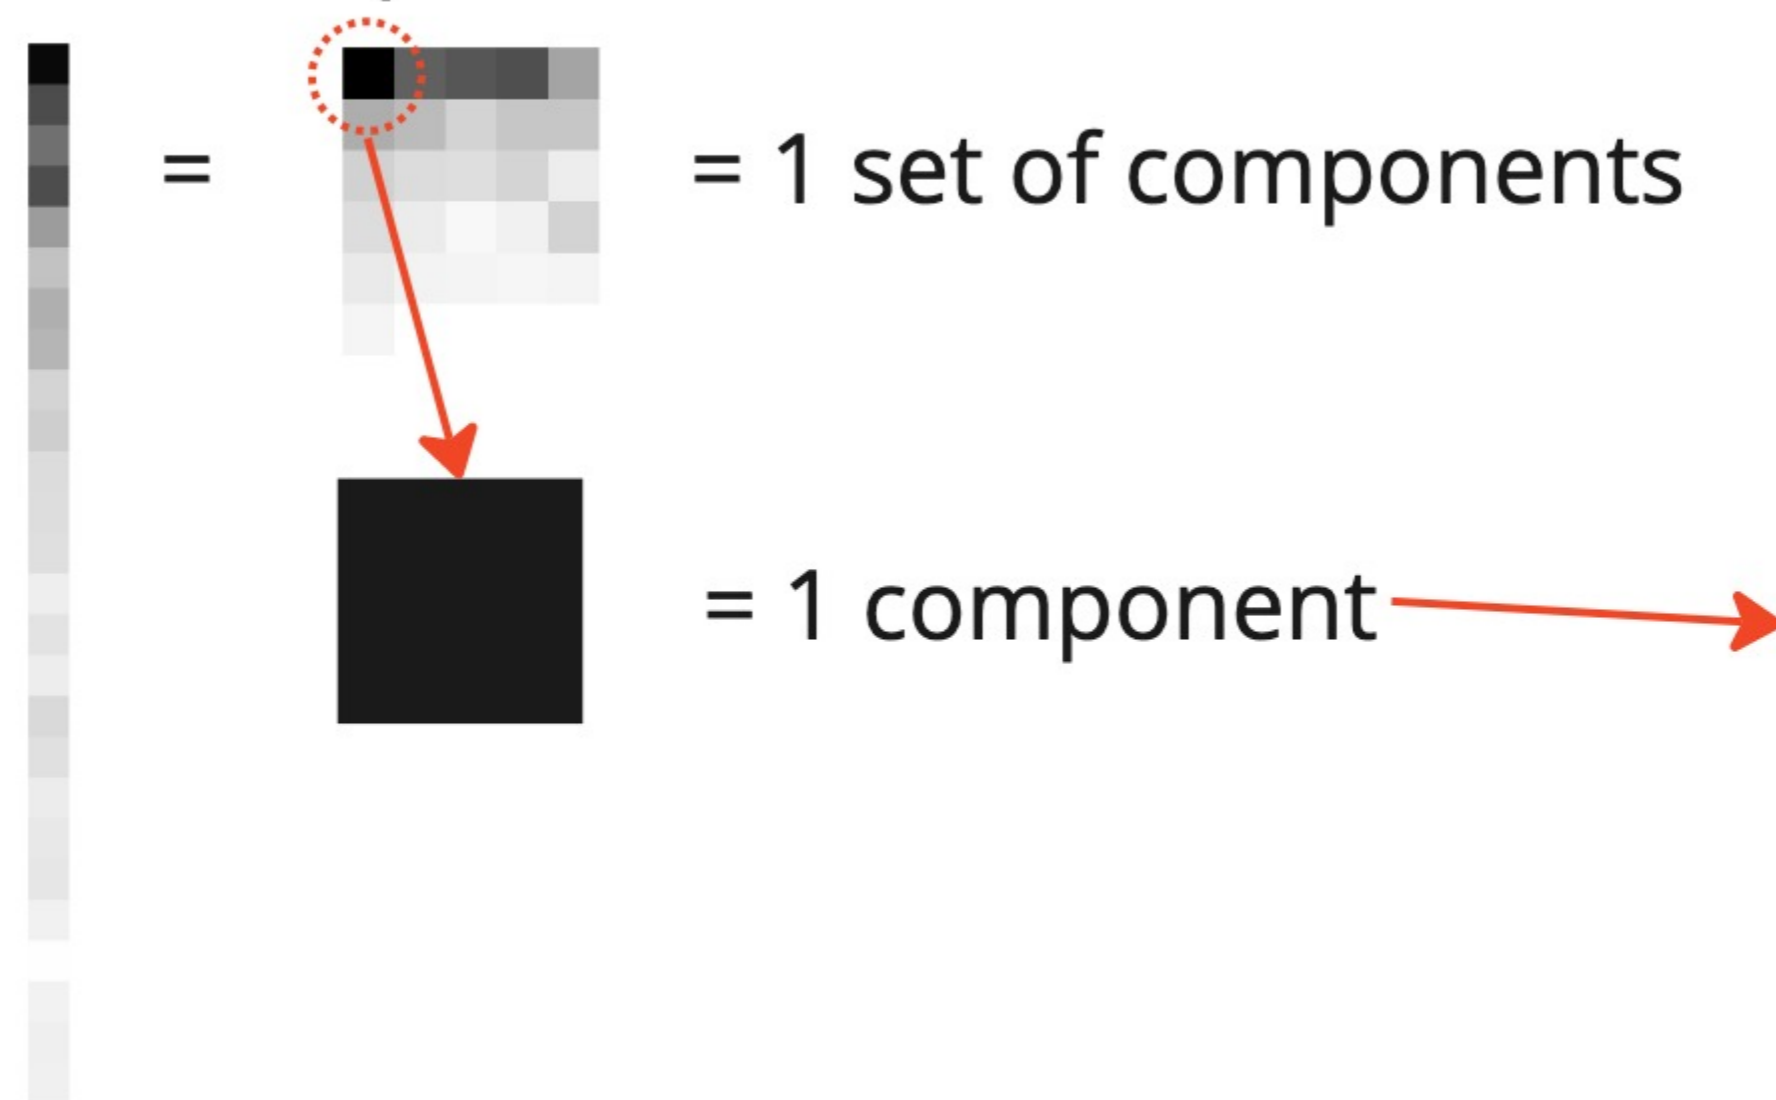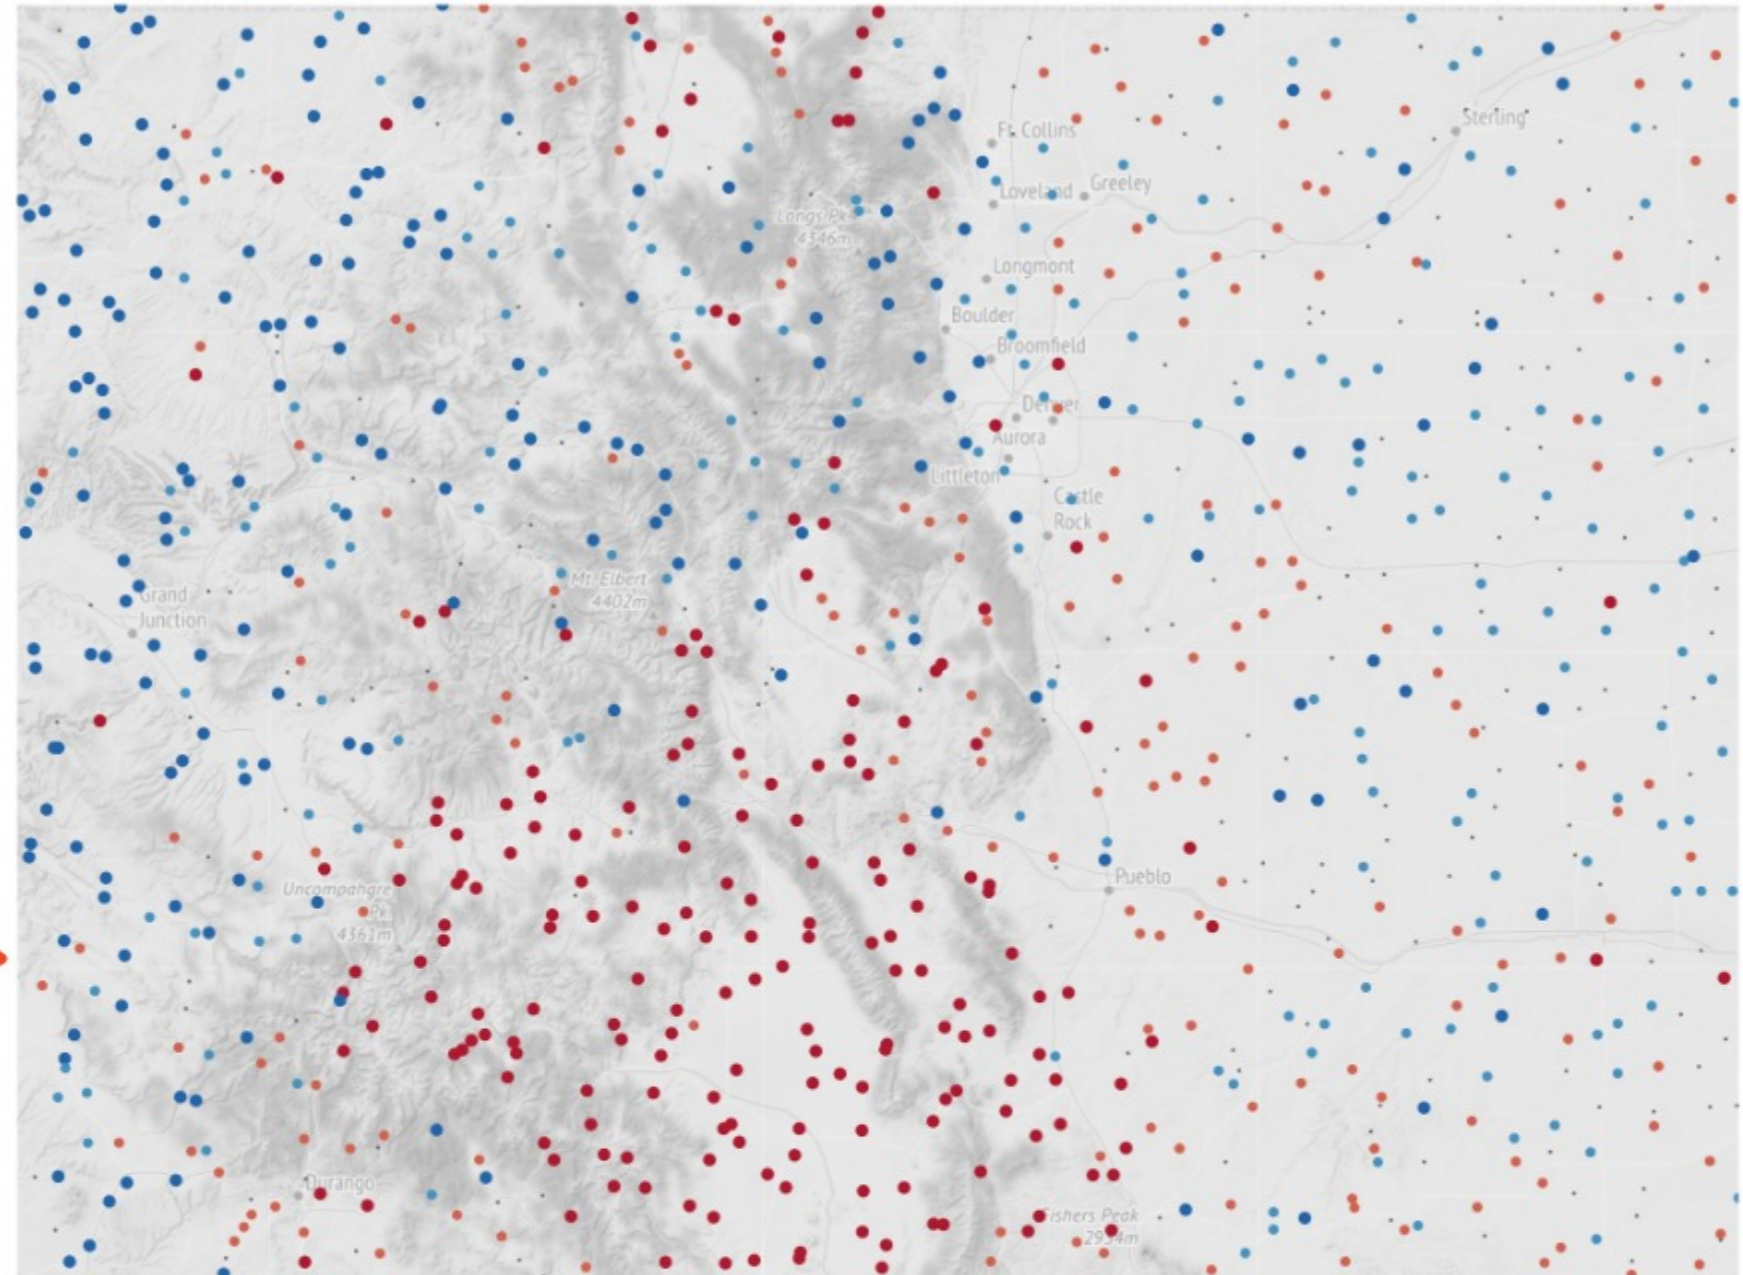

**color (dark is more)**

= spatial autocorrelation (Moran's I)

~ = how clustered are high/low values

~ = how "good" is the component

**color (red is high, blue is low)**

= quintiles of component value

*not* related to red/blue color in  
Discrepancy Dendrogram!

# SNSS Veneto Dataset

- Variables: unmixing matrix **w**, kernels **k**, regionalizations **r**
- 6 kernels x 7 regionalizations = 42 combinations
- Dissimilarity measures  $d(., .)$ :
  - **w**: MD Index
  - **r**: Percentage of location pairs that have unequal relation (in same region or not)
  - **k**: Norm of difference of the spatial kernel matrices

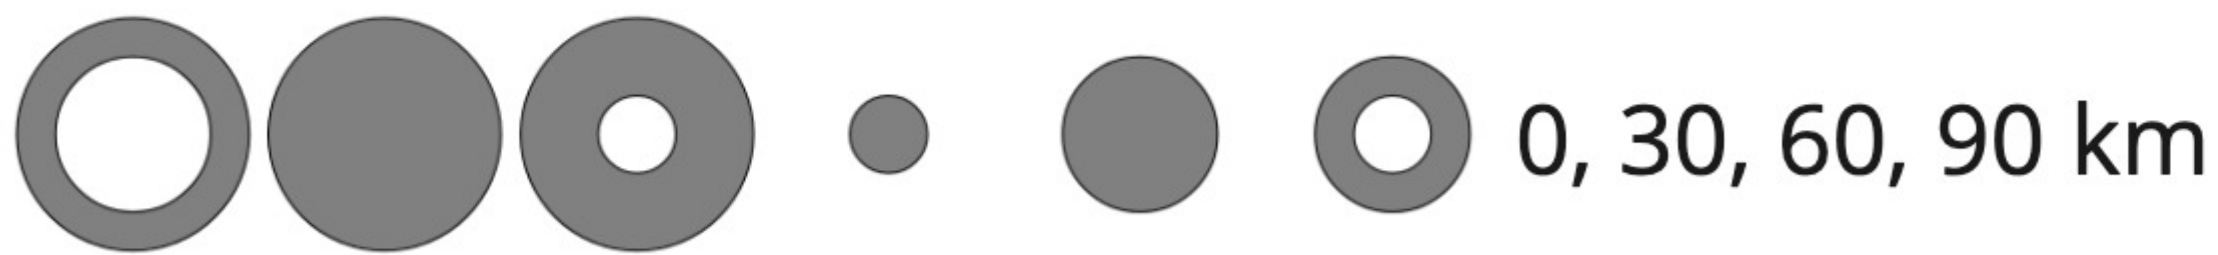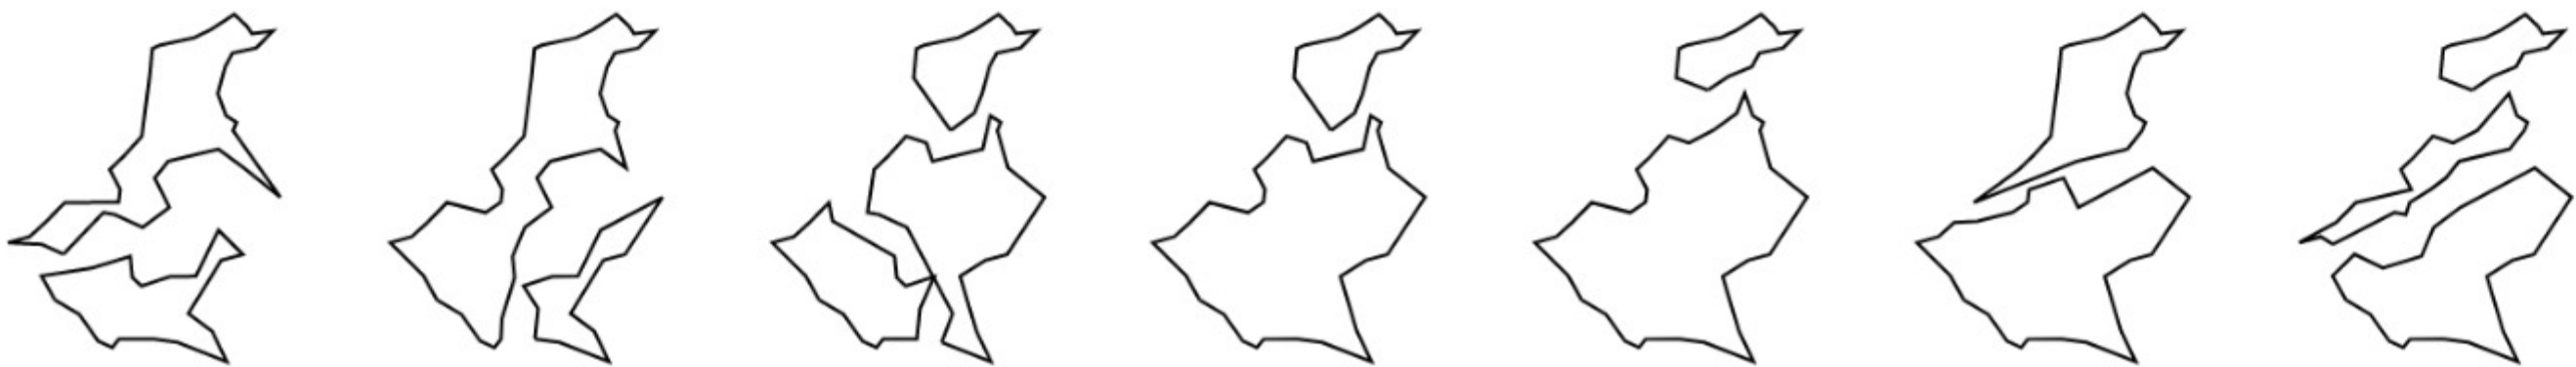

# SNSS Veneto Dataset

- Output visualization:

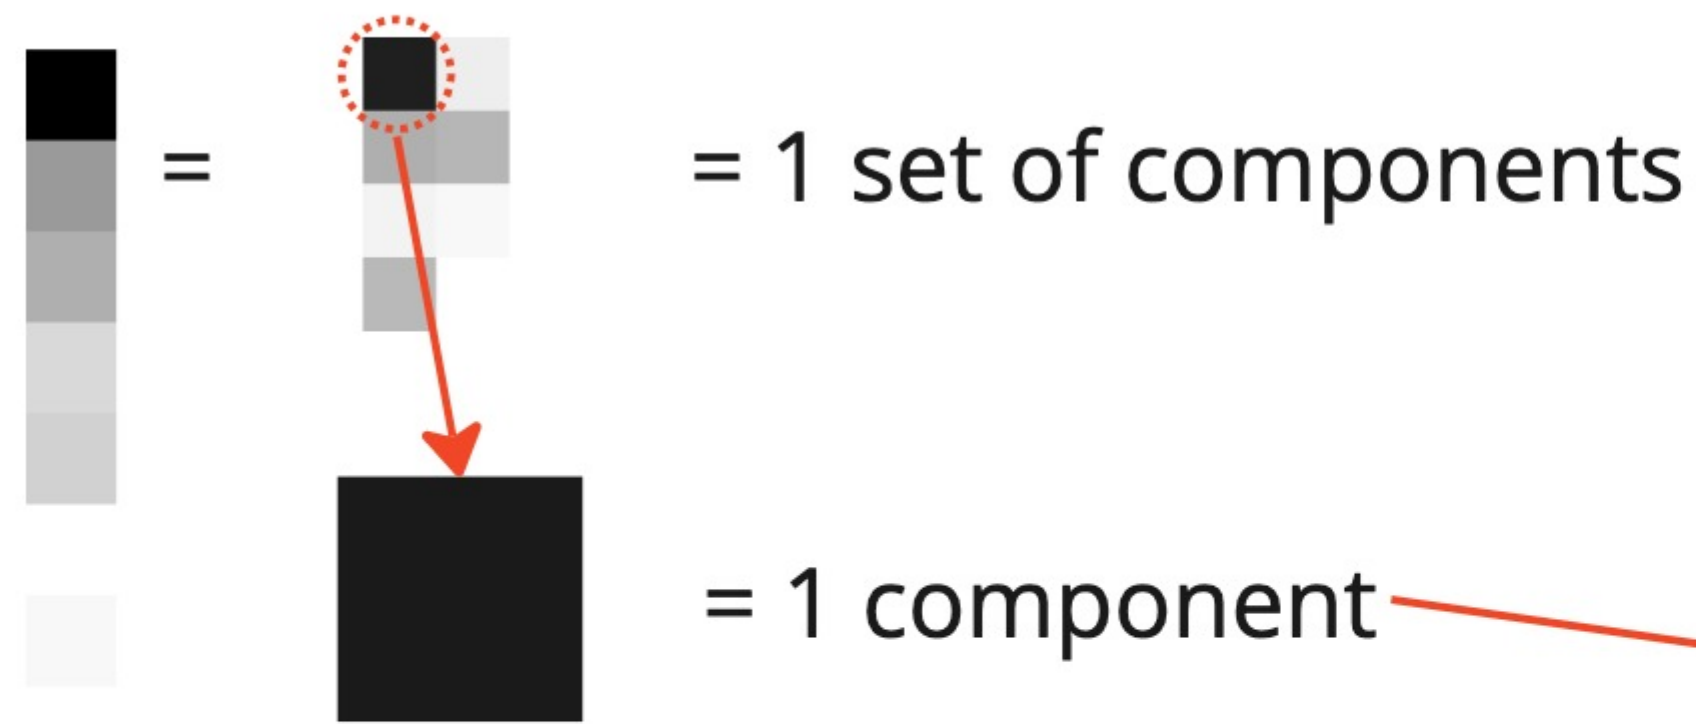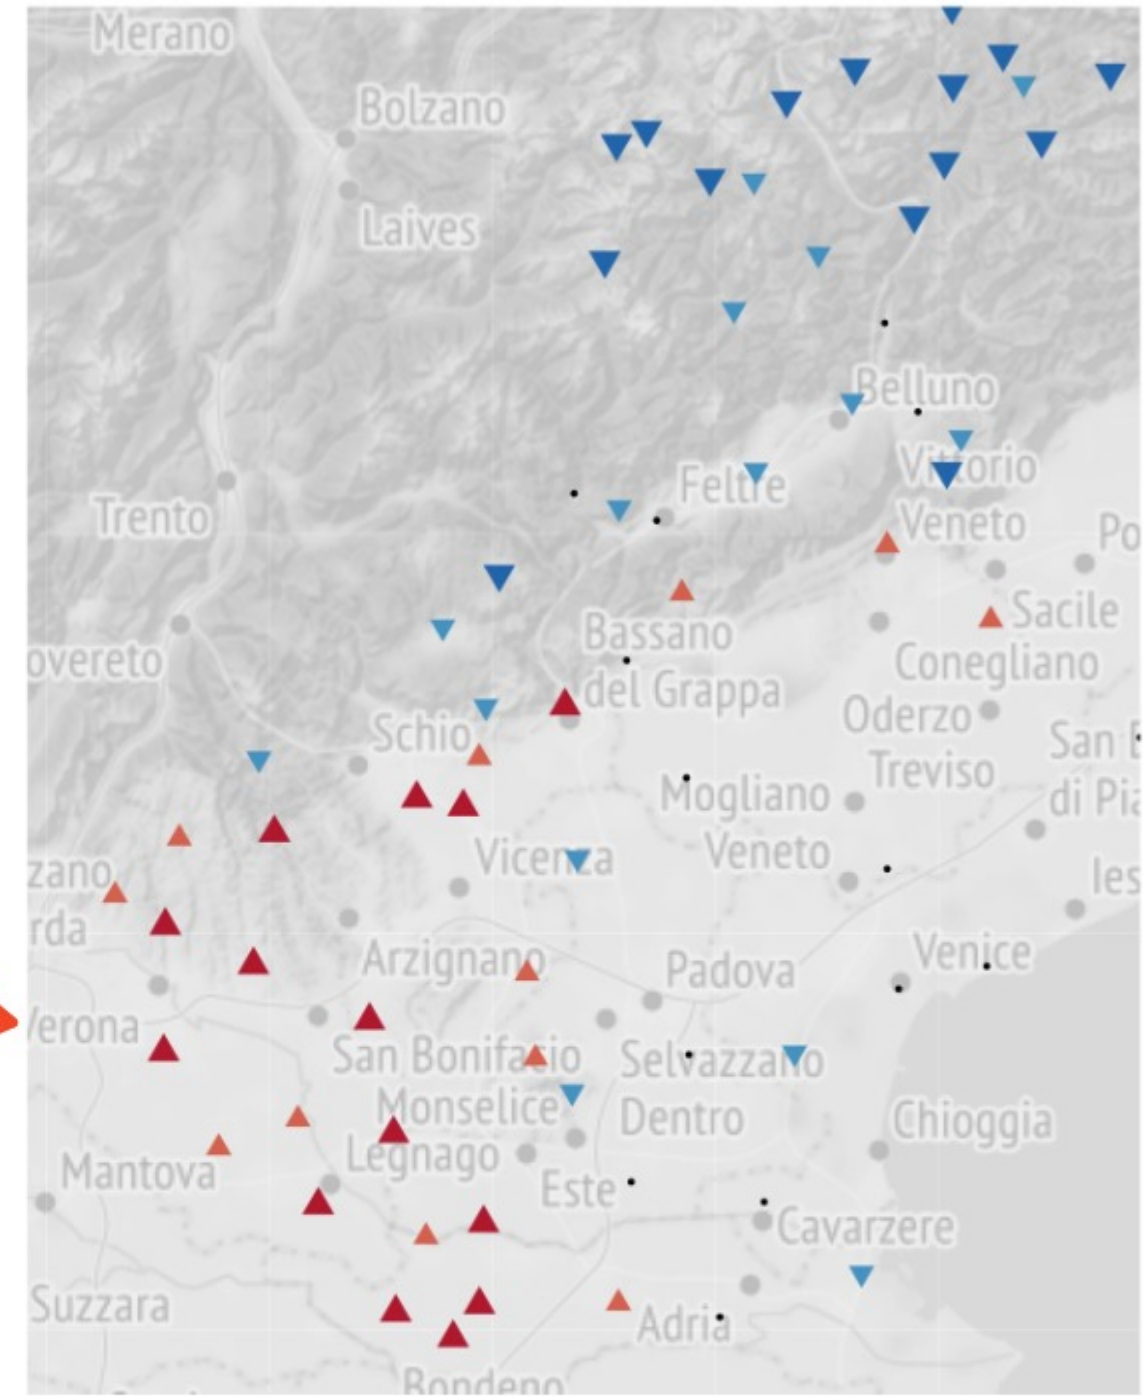

**color (dark is more)**

= spatial autocorrelation (Moran's I)  
~ = how clustered are high/low values  
~ = how "good" is the component

**color (red is high, blue is low)**

= quintiles of component value  
*not* related to red/blue color in  
Discrepancy Dendrogram!

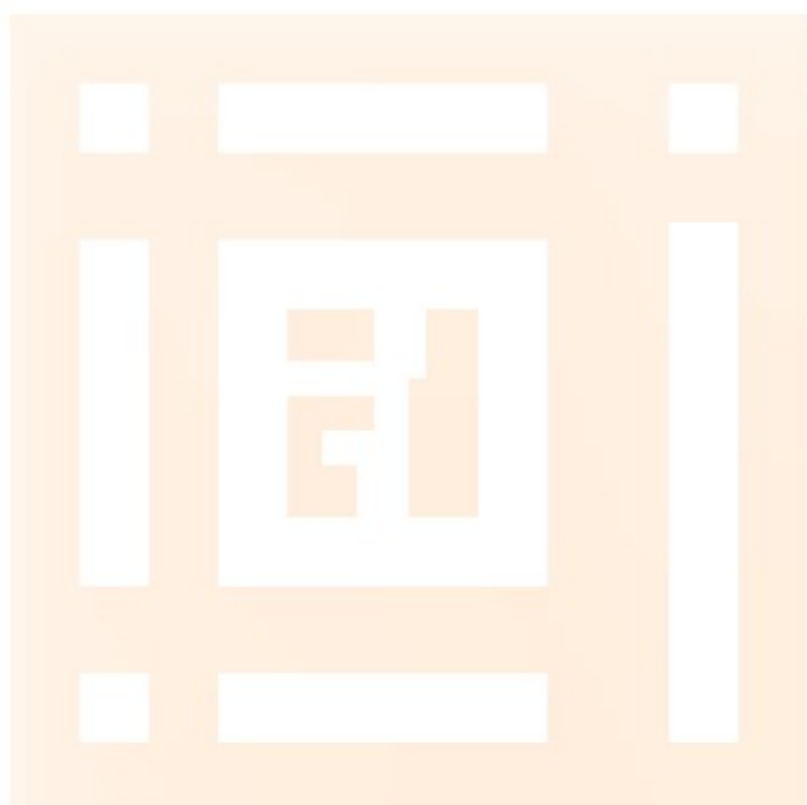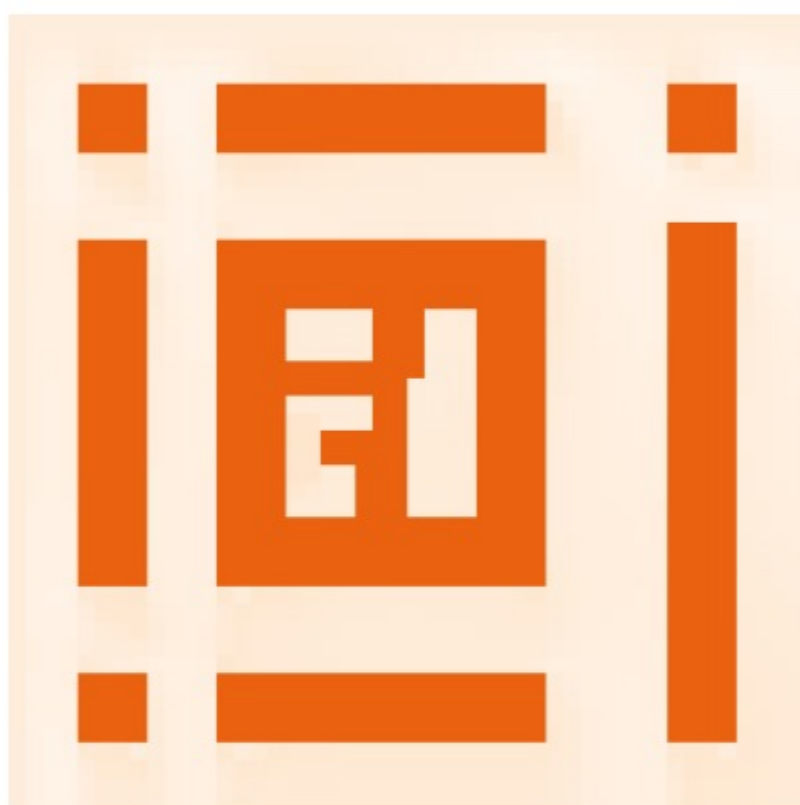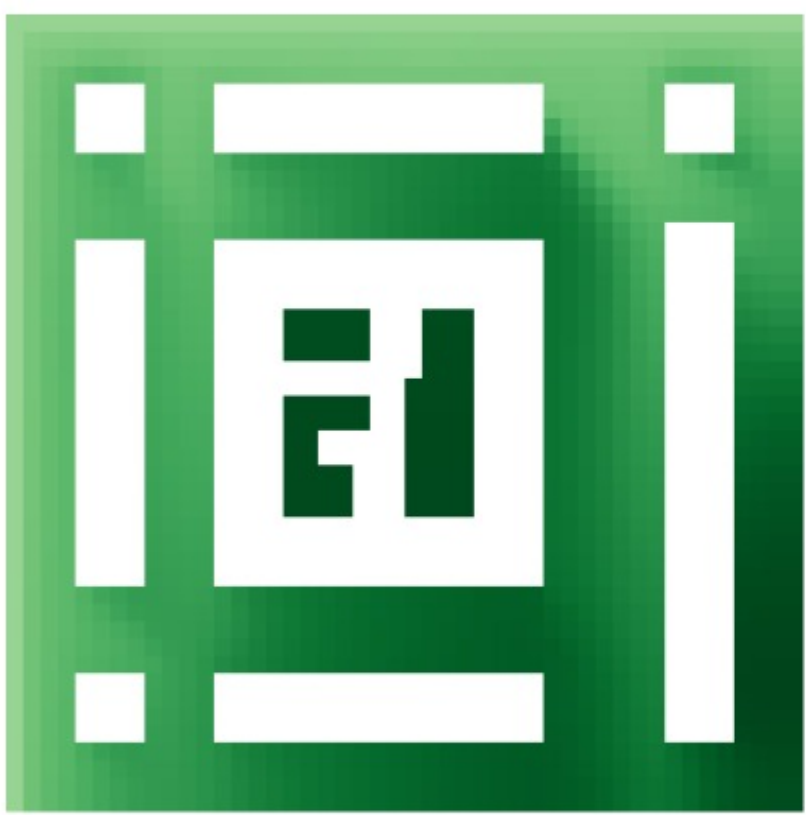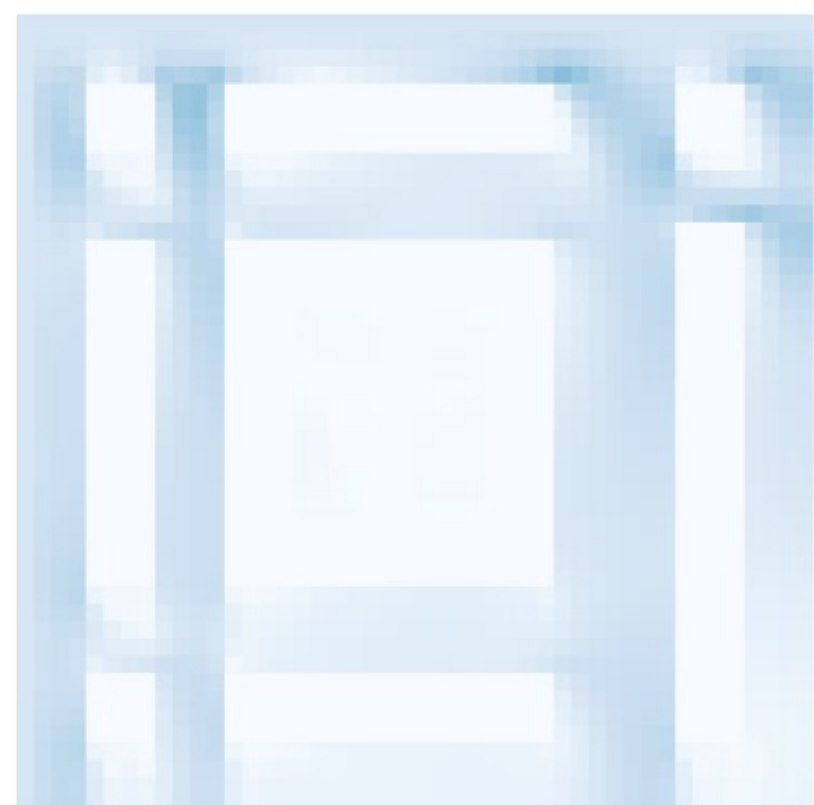

Supplement: Supplementary file 1 [file study-intro.pdf]
