# Supplementary material for: Data Type Agnostic Visual Sensitivity Analysis
Source: arXiv:2309.03580 source file (2023-09-07)
Supplement: Supplementary file 2 [file ice-t.pdf]

| ICET | Question | Score | Question | Score_mean | Score_stdev | ICET | Score_mean | Score_stdev |
|------|----------|-------|----------|------------|-------------|------|------------|-------------|
| 1    | 1        | 7     | 1        | 6.40       | 0.89        | 1    | 6.26       | 1.06        |
| 1    | 2        | 7     | 2        | 5.80       | 1.79        | 2    | 6.08       | 0.91        |
| 1    | 3        | 7     | 3        | 6.60       | 0.55        | 3    | 5.32       | 1.45        |
| 1    | 4        | 7     | 4        | 6.25       | 0.50        | 4    | 5.11       | 2.03        |
| 1    | 5        | 7     | 5        | 5.80       | 1.64        |      |            |             |
| 1    | 6        | 7     | 6        | 6.60       | 0.89        |      |            |             |
| 1    | 7        | 5     | 7        | 6.40       | 0.89        | 1-4  | 5.83       | 1.50        |
| 1    | 8        | 7     | 8        | 6.25       | 0.96        |      |            |             |
| 2    | 9        | 7     | 9        | 5.80       | 1.30        |      |            |             |
| 2    | 10       | 6     | 10       | 6.00       | 1.00        |      |            |             |
| 2    | 11       | 7     | 11       | 6.40       | 0.89        |      |            |             |
| 2    | 12       | 6     | 12       | 6.20       | 0.84        |      |            |             |
| 2    | 13       | 7     | 13       | 6.00       | 0.71        |      |            |             |
| 3    | 14       | 5     | 14       | 4.80       | 1.10        |      |            |             |
| 3    | 15       | 7     | 15       | 6.20       | 0.84        |      |            |             |
| 3    | 16       | 7     | 16       | 5.00       | 1.83        |      |            |             |
| 3    | 17       | 7     | 17       | 5.20       | 1.92        |      |            |             |
| 4    | 18       | 7     | 18       | 6.60       | 0.55        |      |            |             |
| 4    | 19       | 7     | 19       | 6.50       | 0.58        |      |            |             |
| 4    | 20       | 4     | 20       | 4.25       | 1.71        |      |            |             |
| 4    | 21       | 1     | 21       | 3.20       | 2.17        |      |            |             |
| 1    | 1        | 7     |          |            |             |      |            |             |
| 1    | 2        | 7     |          |            |             |      |            |             |
| 1    | 3        | 7     |          |            |             |      |            |             |
| 1    | 4        | NA    |          |            |             |      |            |             |
| 1    | 5        | 6     |          |            |             |      |            |             |
| 1    | 6        | 7     |          |            |             |      |            |             |
| 1    | 7        | 6     |          |            |             |      |            |             |
| 1    | 8        | 7     |          |            |             |      |            |             |
| 2    | 9        | 5     |          |            |             |      |            |             |
| 2    | 10       | 7     |          |            |             |      |            |             |
| 2    | 11       | 6     |          |            |             |      |            |             |
| 2    | 12       | 5     |          |            |             |      |            |             |
| 2    | 13       | 6     |          |            |             |      |            |             |
| 3    | 14       | 3     |          |            |             |      |            |             |
| 3    | 15       | 6     |          |            |             |      |            |             |
| 3    | 16       | 6     |          |            |             |      |            |             |
| 3    | 17       | 2     |          |            |             |      |            |             |
| 4    | 18       | 6     |          |            |             |      |            |             |
| 4    | 19       | 6     |          |            |             |      |            |             |
| 4    | 20       | 2     |          |            |             |      |            |             |
| 4    | 21       | 6     |          |            |             |      |            |             |
| 1    | 1        | 6     |          |            |             |      |            |             |
| 1    | 2        | 5     |          |            |             |      |            |             |
| 1    | 3        | 7     |          |            |             |      |            |             |
| 1    | 4        | 6     |          |            |             |      |            |             |
| 1    | 5        | 3     |          |            |             |      |            |             |
| 1    | 6        | 7     |          |            |             |      |            |             |
| 1    | 7        | 7     |          |            |             |      |            |             |
| 1    | 8        | 5     |          |            |             |      |            |             |
| 2    | 9        | 6     |          |            |             |      |            |             |
| 2    | 10       | 5     |          |            |             |      |            |             |
| 2    | 11       | 5     |          |            |             |      |            |             |
| 2    | 12       | 6     |          |            |             |      |            |             |

| Legend      |                                                                                                                  |
|-------------|------------------------------------------------------------------------------------------------------------------|
| Col.        | Meaning                                                                                                          |
| ICET        | ICE-T component. 1=insight, 2=time, 3=essence, 4=confidence                                                      |
| Question    | question id, in same order as in visvalue survey pdf <a href="https://visvalue.github.io">visvalue.github.io</a> |
| Score       | participant score                                                                                                |
| Score_mean  | mean of score without NA                                                                                         |
| Score_stdev | standard deviation of score without NA                                                                           |

| ICET | Question | Score | Question | Score_mean | Score_stdev | ICET | Score_mean | Score_stdev |
|------|----------|-------|----------|------------|-------------|------|------------|-------------|
| 2    | 13       | 6     |          |            |             |      |            |             |
| 3    | 14       | 6     |          |            |             |      |            |             |
| 3    | 15       | 5     |          |            |             |      |            |             |
| 3    | 16       | 4     |          |            |             |      |            |             |
| 3    | 17       | 6     |          |            |             |      |            |             |
| 4    | 18       | 7     |          |            |             |      |            |             |
| 4    | 19       | 6     |          |            |             |      |            |             |
| 4    | 20       | 6     |          |            |             |      |            |             |
| 4    | 21       | 5     |          |            |             |      |            |             |
| 1    | 1        | 5     |          |            |             |      |            |             |
| 1    | 2        | 3     |          |            |             |      |            |             |
| 1    | 3        | 6     |          |            |             |      |            |             |
| 1    | 4        | 6     |          |            |             |      |            |             |
| 1    | 5        | 6     |          |            |             |      |            |             |
| 1    | 6        | 5     |          |            |             |      |            |             |
| 1    | 7        | 7     |          |            |             |      |            |             |
| 1    | 8        | NA    |          |            |             |      |            |             |
| 2    | 9        | 4     |          |            |             |      |            |             |
| 2    | 10       | 5     |          |            |             |      |            |             |
| 2    | 11       | 7     |          |            |             |      |            |             |
| 2    | 12       | 7     |          |            |             |      |            |             |
| 2    | 13       | 5     |          |            |             |      |            |             |
| 3    | 14       | 5     |          |            |             |      |            |             |
| 3    | 15       | 6     |          |            |             |      |            |             |
| 3    | 16       | 3     |          |            |             |      |            |             |
| 3    | 17       | 5     |          |            |             |      |            |             |
| 4    | 18       | 6     |          |            |             |      |            |             |
| 4    | 19       | NA    |          |            |             |      |            |             |
| 4    | 20       | 5     |          |            |             |      |            |             |
| 4    | 21       | 2     |          |            |             |      |            |             |
| 1    | 1        | 7     |          |            |             |      |            |             |
| 1    | 2        | 7     |          |            |             |      |            |             |
| 1    | 3        | 6     |          |            |             |      |            |             |
| 1    | 4        | 6     |          |            |             |      |            |             |
| 1    | 5        | 7     |          |            |             |      |            |             |
| 1    | 6        | 7     |          |            |             |      |            |             |
| 1    | 7        | 7     |          |            |             |      |            |             |
| 1    | 8        | 6     |          |            |             |      |            |             |
| 2    | 9        | 7     |          |            |             |      |            |             |
| 2    | 10       | 7     |          |            |             |      |            |             |
| 2    | 11       | 7     |          |            |             |      |            |             |
| 2    | 12       | 7     |          |            |             |      |            |             |
| 2    | 13       | 6     |          |            |             |      |            |             |
| 3    | 14       | 5     |          |            |             |      |            |             |
| 3    | 15       | 7     |          |            |             |      |            |             |
| 3    | 16       | NA    |          |            |             |      |            |             |
| 3    | 17       | 6     |          |            |             |      |            |             |
| 4    | 18       | 7     |          |            |             |      |            |             |
| 4    | 19       | 7     |          |            |             |      |            |             |
| 4    | 20       | NA    |          |            |             |      |            |             |
| 4    | 21       | 2     |          |            |             |      |            |             |
